# Supplementary material for: Correlated interaction effects in an anisotropic flat band fermion system
Source: arXiv:2412.13980 ancillary file (2024-12-18)
Supplement: Supplementary file 1 [file Supplement.pdf]

# Supplementary Materials for "Correlated interaction effects in an anisotropic flat band fermion system"

Jing-Rong Wang[1,*] and Chang-Jin Zhang[1,2,†]

[1]High Magnetic Field Laboratory of Anhui Province, Chinese Academy of Sciences, Hefei 230031, China

[2]Institute of Physical Science and Information Technology, Anhui University, Hefei 230601, China

## I. POLARIZATION FUNCTION

The propagator of fermions is expressed as by

$$G_0(\omega,\mathbf{k}) = \frac{1}{-i\omega + v_x k_x\sigma_1 + d_y k_y^3\sigma_2}. \tag{1}$$

The polarization is defined as

$$\Pi(\Omega,\mathbf{q}) \;=\; -\int\frac{d\omega}{2\pi}\int\frac{d^2\mathbf{k}}{(2\pi)^2}\mathrm{Tr}\left[G_0(\omega,\mathbf{k})G_0\left(\omega+\Omega,\mathbf{k}+\mathbf{q}\right)\right]. \tag{2}$$

Substituting the fermion propagator, we get

$$\Pi(\Omega,\mathbf{q}) \;=\; 2\int\frac{d\omega}{2\pi}\int\frac{d^2\mathbf{k}}{(2\pi)^2}\frac{\omega\left(\omega+\Omega\right) - v_x^2 k_x\left(k_x+q_x\right) - d_y^2 k_y^3\left(k_y+q_y\right)^3}{\left[\omega^2 + v_x^2k_x^2 + d_y^2k_y^6\right]\left[\left(\omega+\Omega\right)^2 + v_x^2\left(k_x+q_x\right)^2 + d_y^2\left(k_y+q_y\right)^6\right]}. \tag{3}$$

Using the Ferynman parametrization

$$\frac{1}{AB} = \int_0^1 dx\frac{1}{\left[xA+(1-x)B\right]^2}, \tag{4}$$

we obtain

$$\begin{aligned}\Pi(\Omega,\mathbf{q}) \;=&\; 2\int_0^1 dx\int\frac{d\omega}{2\pi}\int\frac{dk_x}{2\pi}\int\frac{dk_y}{2\pi}\\ &\times\frac{\omega\left(\omega+\Omega\right) - v_x^2k_x\left(k_x+q_x\right) - d_y^2k_y^3\left(k_y+q_y\right)^3}{\left[\left(\omega+x\Omega\right)^2 + v_x^2\left(k_x+xq_x\right)^2 + x(1-x)\Omega^2 + x(1-x)v_x^2q_x^2 + (1-x)d_y^2k_y^6 + xd_y^2\left(k_y+q_y\right)^6\right]^2}.\end{aligned} \tag{5}$$

Adopting the transformations,

$$\omega \;\to\; \omega - x\Omega, \tag{6}$$

$$k_x \;\to\; k_x - xq_x, \tag{7}$$

we arrive

$$\begin{aligned}\Pi(\Omega,\mathbf{q}) \;=&\; 2\int_0^1 dx\int\frac{dk_y}{2\pi}\int\frac{d\omega}{2\pi}\int\frac{dk_x}{2\pi}\\ &\times\frac{\omega^2 - v_x^2k_x^2 - x\left(1-x\right)\Omega^2 + x\left(1-x\right)v_x^2q_x^2 - d_y^2k_y^3\left(k_y+q_y\right)^3}{\left[\omega^2 + v_x^2k_x^2 + x(1-x)\Omega^2 + x(1-x)v_x^2q_x^2 + (1-x)d_y^2k_y^6 + xd_y^2\left(k_y+q_y\right)^6\right]^2}.\end{aligned} \tag{8}$$

---

*Corresponding author: wangjr@hmfl.ac.cn

†Corresponding author: zhangcj@hmfl.ac.cn

Utilizing the transformations

$$q_x \to \frac{q_x}{v_x}, \qquad k_x \to \frac{k_x}{v_x}, \qquad q_y \to \frac{q_y}{d_y^{\frac{1}{3}}}, \qquad k_y \to \frac{k_y}{d_y^{\frac{1}{3}}}, \tag{9}$$

the polarization can be further written as

$$\begin{aligned}\Pi(\Omega, \frac{q_x}{v_x}, \frac{q_y}{d_y^{\frac{1}{3}}}) &= \frac{2}{v_x d_y^{\frac{1}{3}}} \int_0^1 dx \int \frac{dk_y}{2\pi} \int \frac{d\omega}{2\pi} \int \frac{dk_x}{2\pi} \\ &\times \frac{\omega^2 - k_x^2 - x(1-x)\Omega^2 + x(1-x)q_x^2 - k_y^3 (k_y+q_y)^3}{\left[\omega^2 + k_x^2 + x(1-x)\Omega^2 + x(1-x)q_x^2 + (1-x)k_y^6 + x(k_y+q_y)^6\right]^2}.\end{aligned} \tag{10}$$

Let

$$K = (\omega, k_x), \tag{11}$$

the polarization can be expressed by

$$\begin{aligned}\Pi(\Omega, \frac{q_x}{v_x}, \frac{q_y}{d_y^{\frac{1}{3}}}) &= \frac{2}{v_x d_y^{\frac{1}{3}}} \int_0^1 dx \int \frac{dk_y}{2\pi} \left\{ \int \frac{d^2K}{(2\pi)^2} \frac{K^2}{\left[K^2 + x(1-x)\Omega^2 + x(1-x)q_x^2 + (1-x)k_y^6 + x(k_y+q_y)^6\right]^2} \right. \\ &- \int \frac{d^2K}{(2\pi)^2} \frac{1}{K^2 + x(1-x)\Omega^2 + x(1-x)q_x^2 + (1-x)k_y^6 + x(k_y+q_y)^6} \\ &+ \left[2x(1-x)q_x^2 - k_y^3(k_y+q_y)^3 + (1-x)k_y^6 + x(k_y+q_y)^6\right] \\ &\left. \times \int \frac{d^2K}{(2\pi)^2} \frac{1}{\left[K^2 + x(1-x)\Omega^2 + x(1-x)q_x^2 + (1-x)k_y^6 + x(k_y+q_y)^6\right]^2} \right\}.\end{aligned} \tag{12}$$

Using the formula

$$\int \frac{d^dK}{(2\pi)^d} \frac{1}{(K^2+\Delta)^n} = \frac{1}{(4\pi)^{d/2}} \frac{\Gamma(n-d/2)}{\Gamma(n)} \frac{1}{\Delta^{n-d/2}}, \tag{13}$$

$$\int \frac{d^dK}{(2\pi)^d} \frac{K^2}{(K^2+\Delta)^n} = \frac{1}{(4\pi)^{d/2}} \frac{d}{2} \frac{\Gamma(n-\frac{d}{2}-1)}{\Gamma(n)} \frac{1}{\Delta^{n-d/2-1}}, \tag{14}$$

we get

$$\Pi(\Omega, \frac{q_x}{v_x}, \frac{q_y}{d_y^{\frac{1}{3}}}) = \frac{1}{4\pi^2 v_x d_y^{\frac{1}{3}}} \int_0^1 dx \int dk_y \frac{2x(1-x)q_x^2 - k_y^3(k_y+q_y)^3 + (1-x)k_y^6 + x(k_y+q_y)^6}{x(1-x)\Omega^2 + x(1-x)q_x^2 + (1-x)k_y^6 + x(k_y+q_y)^6}. \tag{15}$$

### A. The limit $q_y = 0$

In the limit $q_y = 0$, we have

$$\Pi(\Omega, \frac{q_x}{v_x}, 0) = \frac{1}{2\pi^2 v_x d_y^{\frac{1}{3}}} q_x^2 \int_0^1 dx x(1-x) \int_{-\infty}^{+\infty} dk_y \frac{1}{x(1-x)(\Omega^2+q_x^2) + k_y^6}. \tag{16}$$

Performing the integrations of $k_y$ and $x$, we get

$$\begin{aligned}\Pi(\Omega, \frac{q_x}{v_x}, 0) &= \frac{1}{3\pi v_x d_y^{\frac{1}{3}}} \frac{q_x^2}{(\Omega^2+q_x^2)^{\frac{5}{6}}} \int_0^1 dx x^{\frac{1}{6}} (1-x)^{\frac{1}{6}} \\ &= c_1 \frac{1}{v_x d_y^{\frac{1}{3}}} \frac{q_x^2}{(\Omega^2+q_x^2)^{\frac{5}{6}}},\end{aligned} \tag{17}$$

where

$$c_1 = \frac{\Gamma\left(\frac{1}{6}\right)}{24\cdot 2^{\frac{1}{3}}\sqrt{\pi}\Gamma\left(\frac{2}{3}\right)}. \tag{18}$$

### B. $\Omega = 0$ and $q_x = 0$

Assuming $\Omega = q_x = 0$, we notice that

$$\begin{aligned}\Pi(0,0,\frac{q_y}{d_y^{\frac{1}{3}}}) &= \frac{1}{4\pi^2 v_x d_y^{\frac{1}{3}}}\int dk_y \int_0^1 dx \left[1 - \frac{k_y^3\left(k_y+q_y\right)^3}{(1-x)k_y^6 + x\left(k_y+q_y\right)^6}\right] \\ &= \frac{1}{4\pi^2 v_x d_y^{\frac{1}{3}}}\int_{-\infty}^{+\infty} dk_y \left[1 - \frac{k_y^3\left(k_y+q_y\right)^3}{\left[\left(k_y+q_y\right)^6 - k_y^6\right]}\ln\left(\frac{\left(k_y+q_y\right)^6}{k_y^6}\right)\right].\end{aligned} \tag{19}$$

$\Pi(0,0,\frac{q_y}{d_y^{\frac{1}{3}}})$ can be further written as

$$\Pi(0,0,\frac{q_y}{d_y^{\frac{1}{3}}}) = \frac{1}{4\pi^2 v_x d_y^{\frac{1}{3}}}|q_y|\int_{-\infty}^{+\infty} dx \left[1 - \frac{x^3\left(x+1\right)^3}{\left[\left(x+1\right)^6 - x^6\right]}\ln\left(\frac{\left(x+1\right)^6}{x^6}\right)\right]. \tag{20}$$

Using the formula

$$\int_{-\infty}^{+\infty} dx \left[1 - \frac{x^3\left(x+1\right)^3}{\left[\left(x+1\right)^6 - x^6\right]}\ln\left(\frac{\left(x+1\right)^6}{x^6}\right)\right] = \frac{17\pi^2}{36}, \tag{21}$$

we obtain

$$\Pi(0,0,\frac{q_y}{d_y^{\frac{1}{3}}}) = c_2\frac{1}{v_x d_y^{\frac{1}{3}}}|q_y|, \tag{22}$$

where

$$c_2 = \frac{17}{144}. \tag{23}$$

### C. $\Omega >> d_y q_y^3$ and $q_x = 0$

In the limit $\Omega >> d_y q_y^3$ and $q_x = 0$, we have

$$\begin{aligned}\Pi(\Omega,0,\frac{q_y}{d_y^{\frac{1}{3}}}) &= \frac{1}{4\pi^2 v_x d_y^{\frac{1}{3}}}\int_0^1 dx \int dk_y \frac{-k_y^3\left(k_y+q_y\right)^3 + (1-x)k_y^6 + x\left(k_y+q_y\right)^6}{x(1-x)\Omega^2 + (1-x)k_y^6 + x\left(k_y+q_y\right)^6} \\ &= \frac{1}{4\pi^2 v_x d_y^{\frac{1}{3}}}q_y^2\int_0^1 dx 3\left(5x-1\right)\int_{-\infty}^{+\infty} dk_y \frac{k_y^4}{\left[x(1-x)\Omega^2 + k_y^6\right]} \\ &\quad + \frac{1}{4\pi^2 v_x d_y^{\frac{1}{3}}}q_y^2\int_0^1 dx 18x\left(1-2x\right)\int_{-\infty}^{+\infty} dk_y \frac{k_y^{10}}{\left[x(1-x)\Omega^2 + k_y^6\right]^2}.\end{aligned} \tag{24}$$

Let

$$k_y = \left[x(1-x)\Omega^2\right]^{\frac{1}{6}} y, \tag{25}$$

the polarization can be written as

$$\Pi(\Omega,0,\frac{q_y}{d_y^{\frac{1}{3}}}) = \frac{1}{2\pi v_x d_y^{\frac{1}{3}}}\frac{q_y^2}{\left(\Omega^2\right)^{\frac{1}{6}}}\int_0^1 dx \frac{10x\left(1-x\right)-1}{\left[x(1-x)\right]^{\frac{1}{6}}}. \tag{26}$$

Employing

$$\int_0^1 dx \frac{10x(1-x)-1}{[x(1-x)]^{\frac{1}{6}}} = \frac{9\sqrt{\pi}\Gamma\left(\frac{5}{6}\right)}{16\cdot 2^{\frac{2}{3}}\Gamma\left(\frac{4}{3}\right)}, \tag{27}$$

we obtain

$$\Pi(\Omega, 0, \frac{q_y}{d_y^{\frac{1}{3}}}) = c_3 \frac{1}{v_x d_y^{\frac{1}{3}}} \frac{q_y^2}{(\Omega^2)^{\frac{1}{6}}}, \tag{28}$$

where

$$c_3 = \frac{9\Gamma\left(\frac{5}{6}\right)}{32\cdot 2^{\frac{2}{3}}\sqrt{\pi}\Gamma\left(\frac{4}{3}\right)}. \tag{29}$$

### D. The ansatz for the polarization function

According to the polarization calculated in different limits shown in Eqs. (17), (22), and (28), we find that the polarization can be approximated by the following ansatz

$$\Pi(\Omega, \frac{q_x}{v_x}, \frac{q_y}{d_y^{\frac{1}{3}}}) = \frac{1}{v_x d_y^{\frac{1}{3}}} \left[ \frac{c_1 q_x^2}{\left(\Omega^2 + q_x^2 + \frac{c_3^6}{c_2^6} q_y^6\right)^{\frac{5}{6}}} + \frac{c_3 q_y^2}{\left(\Omega^2 + q_x^2 + \frac{c_3^6}{c_2^6} q_y^6\right)^{\frac{1}{6}}} \right] \tag{30}$$

Using the rescaling relations

$$\frac{q_x}{v_x} \to q_x, \qquad \frac{q_y}{d_y^{\frac{1}{3}}} \to q_y, \tag{31}$$

the polarization can be further written as

$$\Pi(\Omega, q_x, q_y) = \frac{1}{v_x d_y^{\frac{1}{3}}} \left[ \frac{c_1 v_x^2 q_x^2}{\left(\Omega^2 + v_x^2 q_x^2 + \frac{c_3^6}{c_2^6} d_y^2 q_y^6\right)^{\frac{5}{6}}} + \frac{c_3 d_y^{\frac{2}{3}} q_y^2}{\left(\Omega^2 + v_x^2 q_x^2 + \frac{c_3^6}{c_2^6} d_y^2 q_y^6\right)^{\frac{1}{6}}} \right]. \tag{32}$$

## II. SELF-ENERGY OF FERMIONS

Firstly, we calculate the fermion self-energy through the bare Coulomb interaction $V_0(\mathbf{q})$, which takes the form

$$V_0(\mathbf{q}) = \frac{2\pi e^2}{\epsilon |\mathbf{q}|}, \tag{33}$$

where $e$ is the electric charge, and $\epsilon$ the dielectric constant. The fermion self-energy can be written as

$$\Sigma(\omega, \mathbf{k}) = \int \frac{d\Omega}{2\pi} \int' \frac{d^2\mathbf{q}}{(2\pi)^2} G_0\left(\omega+\Omega, \mathbf{k}+\mathbf{q}\right) V_0(\Omega, \mathbf{q}), \tag{34}$$

where $\int'$ stands for that a momentum shell will be properly imposed. Substituting the propagator of fermion, we get

$$\Sigma(\omega, \mathbf{k}) = \int \frac{d\Omega}{2\pi} \int' \frac{d^2\mathbf{q}}{(2\pi)^2} \frac{i(\omega+\Omega) + v_x(k_x+q_x)\sigma_1 + d_y(k_y+q_y)^3\sigma_2}{(\omega+\Omega)^2 + v_x^2(k_x+q_x)^2 + d_y^2(k_y+q_y)^6} V_0(\Omega, \mathbf{q}) \tag{35}$$

Expanding to leading terms of $k_x$ and $k_y$, we obtain

$$\Sigma(\omega, \mathbf{k}) = -i\omega\Sigma_0 + v_x k_x \sigma_1 + d_y k_y^3 \sigma_2 + k_y \sigma_2 \Sigma_L. \tag{36}$$

where

$$\Sigma_0 = \int\frac{d\Omega}{2\pi}\int'\frac{d^2\mathbf{q}}{(2\pi)^2}\frac{\Omega^2-v_x^2q_x^2-d_y^2q_y^6}{\left(\Omega^2+v_x^2q_x^2+d_y^2q_y^6\right)^2}V_0(\Omega,\mathbf{q}), \tag{37}$$

$$\Sigma_1 = \int\frac{d\Omega}{2\pi}\int'\frac{d^2\mathbf{q}}{(2\pi)^2}\frac{\Omega^2-v_x^2q_x^2+d_y^2q_y^6}{\left(\Omega^2+v_x^2q_x^2+d_y^2q_y^6\right)^2}V_0(\Omega,\mathbf{q}), \tag{38}$$

$$\Sigma_2 = \int\frac{d\Omega}{2\pi}\int'\frac{d^2\mathbf{q}}{(2\pi)^2}\left[\frac{\Omega^2+v_x^2q_x^2-82d_y^2q_y^6}{\left(\Omega^2+v_x^2q_x^2+d_y^2q_y^6\right)^2}+\frac{288d_y^4q_y^{12}}{\left(\Omega^2+v_x^2q_x^2+d_y^2q_y^6\right)^3}-\frac{216d_y^6q_y^{18}}{\left(\Omega^2+v_x^2q_x^2+d_y^2q_y^6\right)^4}\right]V_0(\Omega,\mathbf{q}), \tag{39}$$

$$\Sigma_L = \int\frac{d\Omega}{2\pi}\int'\frac{d^2\mathbf{q}}{(2\pi)^2}\left[\frac{3d_yq_y^2\left(\Omega^2+v_x^2q_x^2-d_y^2q_y^6\right)}{\left(\Omega^2+v_x^2q_x^2+d_y^2q_y^6\right)^2}\right]V_0(\Omega,\mathbf{q}). \tag{40}$$

We can find that a linear term of $k_y$ is generated dynamically. Accordingly, the fermion velocity along $y$ axis is restored.

## III. DERIVATION OF RG EQUATIONS FOR THE PARAMETERS CONSIDERING BARE COULOMB INTERACTION

### A. Self-energy of fermions

In order to consider the dynamically generated term, we employ the propagator of fermion as following

$$G_0^{new}(\omega,\mathbf{k}) = \frac{1}{-i\omega+v_xk_x\sigma_1+\left(v_yk_y+d_yk_y^3\right)\sigma_2}. \tag{41}$$

The fermion self-energy can be written as

$$\Sigma(\omega,k) = \int\frac{d\Omega}{2\pi}\int'\frac{d^2\mathbf{q}}{(2\pi)^2}G_0^{new}\left(\omega+\Omega,\mathbf{k}+\mathbf{q}\right)V_0(\Omega,\mathbf{q}). \tag{42}$$

Substituting the propagator of fermion, we get

$$\Sigma(\omega,\mathbf{k}) = \int\frac{d\Omega}{2\pi}\int'\frac{d^2\mathbf{q}}{(2\pi)^2}\frac{i\left(\omega+\Omega\right)+v_x\left(k_x+q_x\right)\sigma_1+\left[v_y\left(k_y+q_y\right)+d_y\left(k_y+q_y\right)^3\right]\sigma_2}{\left(\omega+\Omega\right)^2+v_x^2\left(k_x+q_x\right)^2+\left[v_y\left(k_y+q_y\right)+d_y\left(k_y+q_y\right)^3\right]^2}V_0(\Omega,\mathbf{q}). \tag{43}$$

Expanding to the leading terms of $\omega$, $k_x$ and $k_y$, we obtain

$$\Sigma(\omega,\mathbf{k}) = -i\omega\Sigma_0+v_xk_x\sigma_1\Sigma_1+v_yk_y\sigma_2\Sigma_2^a+d_yk_y^3\sigma_2\Sigma_2^b, \tag{44}$$

where

$$\Sigma_0 = \int\frac{d\Omega}{2\pi}\int'\frac{d^2\mathbf{q}}{(2\pi)^2}\frac{\Omega^2-\left(v_x^2q_x^2+v_y^2q_y^2+2v_yd_yq_y^4+d_y^2q_y^6\right)}{\left(\Omega^2+v_x^2q_x^2+v_y^2q_y^2+2v_yd_yq_y^4+d_y^2q_y^6\right)^2}V_0(\Omega,\mathbf{q}), \tag{45}$$

$$\Sigma_1 = \int\frac{d\Omega}{2\pi}\int'\frac{d^2\mathbf{q}}{(2\pi)^2}\frac{\Omega^2-v_x^2q_x^2+v_y^2q_y^2+2v_yd_yq_y^4+d_y^2q_y^6}{\left(\Omega^2+v_x^2q_x^2+v_y^2q_y^2+2v_yd_yq_y^4+d_y^2q_y^6\right)^2}V_0(\Omega,\mathbf{q}), \tag{46}$$

$$\Sigma_2^a = \int\frac{d\Omega}{2\pi}\int'\frac{d^2\mathbf{q}}{(2\pi)^2}\left\{\frac{1+3\frac{d_y}{v_y}q_y^2}{\Omega^2+v_x^2q_x^2+v_y^2q_y^2+2v_yd_yq_y^4+d_y^2q_y^6}\right.$$
$$\left.-\frac{2v_y^2q_y^2+10v_yd_yq_y^4+14d_y^2q_y^6+6\frac{d_y^3}{v_y}q_y^8}{\left(\Omega^2+v_x^2q_x^2+v_y^2q_y^2+2v_yd_yq_y^4+d_y^2q_y^6\right)^2}\right\}V_0(\Omega,\mathbf{q}), \tag{47}$$

$$\Sigma_2^b = \int\frac{d\Omega}{2\pi}\int'\frac{d^2\mathbf{q}}{(2\pi)^2}\left\{\frac{1}{\Omega^2+v_x^2q_x^2+v_y^2q_y^2+2v_yd_yq_y^4+d_y^2q_y^6}\right.$$

$$
\begin{aligned}
&-\frac{\frac{v_y^3}{d_y}+29v_y^2q_y^2+103v_yd_yq_y^4+83d_y^2q_y^6}{\left(\Omega^2+v_x^2q_x^2+v_y^2q_y^2+2v_yd_yq_y^4+d_y^2q_y^6\right)^2} \\
&+\frac{8\frac{v_y^5}{d_y}q_y^2+112v_y^4q_y^4+512v_y^3d_yq_y^6+1008v_y^2d_y^2q_y^8+888v_yd_y^3q_y^{10}+288d_y^4q_y^{12}}{\left(\Omega^2+v_x^2q_x^2+v_y^2q_y^2+2v_yd_yq_y^4+d_y^2q_y^6\right)^3} \\
&-\frac{1}{\left(\Omega^2+v_x^2q_x^2+v_y^2q_y^2+2v_yd_yq_y^4+d_y^2q_y^6\right)^4}\left[8\frac{v_y^7}{d_y}q_y^4+104v_y^6q_y^6+552v_y^5d_yq_y^8+1544v_y^4d_y^2q_y^{10}\right. \\
&\left.+2456v_y^3d_y^3q_y^{12}+2232v_y^2d_y^4q_y^{14}+1080v_yd_y^5q_y^{16}+216d_y^6q_y^{18}\right]\Big\}\, V_0(\Omega,\mathbf{q}). \qquad (48)
\end{aligned}
$$

We employ the RG scheme

$$-\infty<\Omega<+\infty, \qquad (49)$$
$$b\Lambda<|\mathbf{q}|<\Lambda, \qquad (50)$$

where $b=e^{-\ell}$ with $\ell$ being the RG running parameter. Performing direct derivations, we obtain

$$\Sigma_0 = 0, \qquad (51)$$
$$\Sigma_1 = C_1\ell, \qquad (52)$$
$$\Sigma_2^a = C_2^a\ell, \qquad (53)$$
$$\Sigma_2^b = C_2^b\ell, \qquad (54)$$

where

$$C_1 = \frac{\alpha}{4\pi}\int_0^{2\pi}d\varphi\frac{\delta^2\sin^2(\varphi)+2\delta\beta\sin^4(\varphi)+\beta^2\sin^6(\varphi)}{\left[\cos^2(\varphi)+\delta^2\sin^2(\varphi)+2\delta\beta\sin^4(\varphi)+\beta^2\sin^6(\varphi)\right]^{\frac{3}{2}}}, \qquad (55)$$

$$
\begin{aligned}
C_2^a = \frac{\alpha}{4\pi}\int_0^{2\pi}d\varphi\Bigg\{&\frac{1+3\frac{1}{\delta}\beta\sin^2(\varphi)}{\left[\cos^2(\varphi)+\delta^2\sin^2(\varphi)+2\delta\beta\sin^4(\varphi)+\beta^2\sin^6(\varphi)\right]^{\frac{1}{2}}} \\
&-\frac{\delta^2\sin^2(\varphi)+5\delta\beta\sin^4(\varphi)+7\beta^2\sin^6(\varphi)+3\frac{1}{\delta}\beta^3\sin^8(\varphi)}{\left[\cos^2(\varphi)+\delta^2\sin^2(\varphi)+2\delta\beta\sin^4(\varphi)+\beta^2\sin^6(\varphi)\right]^{\frac{3}{2}}}\Bigg\}, \qquad (56)
\end{aligned}
$$

$$
\begin{aligned}
C_2^b = \frac{\alpha}{4\pi}\int_0^{2\pi}d\varphi\Bigg\{&\frac{1}{\left(\cos^2(\varphi)+\delta^2\sin^2(\varphi)+2\delta\beta\sin^4(\varphi)+\beta^2\sin^6(\varphi)\right)^{\frac{1}{2}}} \\
&-\frac{1}{2}\frac{\delta^3\frac{1}{\beta}+29\delta^2\sin^2(\varphi)+103\delta\beta\sin^4(\varphi)+83\beta^2\sin^6(\varphi)}{\left(\cos^2(\varphi)+\delta^2\sin^2(\varphi)+2\delta\beta\sin^4(\varphi)+\beta^2\sin^6(\varphi)\right)^{\frac{3}{2}}} \\
&+\frac{1}{\left(\cos^2(\varphi)+\delta^2\sin^2(\varphi)+2\delta\beta\sin^4(\varphi)+\beta^2\sin^6(\varphi)\right)^{\frac{5}{2}}}\left[3\delta^5\frac{1}{\beta}\sin^2(\varphi)+42\delta^4\sin^4(\varphi)\right. \\
&\left.+192\delta^3\beta\sin^6(\varphi)+378\delta^2\beta^2\sin^8(\varphi)+333\delta\beta^3\sin^{10}(\varphi)+108\beta^4\sin^{12}(\varphi)\right] \\
&-\frac{5}{2}\frac{1}{\left(\cos^2(\varphi)+\delta^2\sin^2(\varphi)+2\delta\beta\sin^4(\varphi)+\beta^2\sin^6(\varphi)\right)^{\frac{7}{2}}}\left[\delta^7\frac{1}{\beta}\sin^4(\varphi)+13\delta^6\sin^6(\varphi)+69\delta^5\beta\sin^8(\varphi)\right. \\
&\left.+193\delta^4\beta^2\sin^{10}(\varphi)+307\delta^3\beta^3\sin^{12}(\varphi)+279\delta^2\beta^4\sin^{14}(\varphi)+135\delta\beta^5\sin^{16}(\varphi)+27\beta^6\sin^{18}(\varphi)\right]\Bigg\}. \qquad (57)
\end{aligned}
$$

The parameters $\alpha$, $\beta$, and $\gamma$ are defined as

$$\alpha = \frac{e^2}{\epsilon v_x}, \qquad (58)$$
$$\beta = \frac{d_y\Lambda^2}{v_x}, \qquad (59)$$
$$\delta = v_y/v_x. \qquad (60)$$

### B. Derivation of RG equations

The action of fermions is

$$S_\psi = \int \frac{d\omega}{2\pi}\frac{dk_x}{2\pi}\frac{dk_y}{2\pi}\psi^\dagger(\omega,\mathbf{k})\left(-i\omega + v_x k_x\sigma_1 + \left(v_y k_y + d_y k_y^3\right)\sigma_2\right)\psi(\omega,\mathbf{k}). \tag{61}$$

Including the fermion self-energy induced by Coulomb interaction, the action becomes

$$\begin{aligned} S_\psi &= \int \frac{d\omega}{2\pi}\frac{dk_x}{2\pi}\frac{dk_y}{2\pi}\psi^\dagger(\omega,\mathbf{k})\left(-i\omega + v_x k_x\sigma_1 + \left(v_y k_y + d_y k_y^3\right)\sigma_2 + \Sigma(\omega,\mathbf{k})\right)\psi(\omega,\mathbf{k}) \\ &\approx \int \frac{d\omega}{2\pi}\frac{dk_x}{2\pi}\frac{dk_y}{2\pi}\bar{\Psi}(\omega,\mathbf{k})\left[-i\omega + v_x k_x\sigma_1 e^{C_1\ell} + \left(v_y k_y e^{C_2^a\ell} + d_y k_y^3 e^{C_2^b\ell}\right)\sigma_2\right]\Psi(\omega,\mathbf{k}). \end{aligned} \tag{62}$$

Utilizing the scaling transformations

$$k_x = k_x' e^{-\ell}, \tag{63}$$
$$k_y = k_y' e^{-\ell}, \tag{64}$$
$$\omega = \omega' e^{-\ell}, \tag{65}$$
$$\psi = \psi' e^{2\ell}, \tag{66}$$
$$v_x = v_x' e^{-C_1\ell}, \tag{67}$$
$$v_y = v_y' e^{-C_2^a\ell}, \tag{68}$$
$$d_y = d_y' e^{\left(2-C_2^b\right)\ell}, \tag{69}$$

the action can be written as

$$S_{\Psi'} = \int \frac{d\omega'}{2\pi}\frac{dk_x'}{2\pi}\frac{dk_y'}{2\pi}\bar{\Psi}'(\omega',\mathbf{k}')\left(-i\omega' + v_x' k_x'\sigma_1 + \left(v_y' k_y' + d_y' k_y'^3\right)\sigma_2\right)\Psi'(\omega',\mathbf{k}'), \tag{70}$$

which recover the original form of the fermion action. From Eqs. (67)-(69) we can get the RG equations for $v_x$, $v_y$ and $d_y$

$$\frac{dv_x}{d\ell} = C_1 v_x, \tag{71}$$
$$\frac{dv_y}{d\ell} = C_2^a v_y, \tag{72}$$
$$\frac{dd_y}{d\ell} = \left(-2 + C_2^b\right) d_y. \tag{73}$$

The RG equations for the parameters $\alpha$, $\beta$, and $\gamma$ are

$$\frac{d\alpha}{d\ell} = -C_1\alpha, \tag{74}$$
$$\frac{d\beta}{d\ell} = \left(-2 - C_1 + C_2^b\right)\beta, \tag{75}$$
$$\frac{d\delta}{d\ell} = \left(C_2^a - C_1\right)\delta. \tag{76}$$

## IV. DERIVATION OF RG EQUATIONS FOR THE PARAMETERS CONSIDERING DRESSED COULOMB INTERACTION

### A. Self-energy of fermions

The dressed long-range Coulomb interaction can be approximately written as

$$V^\star(\Omega,\mathbf{q}) = \frac{1}{V_0^{-1}(|\mathbf{q}|) + F_1\Pi(\Omega,\mathbf{q}) + F_2\Pi_{\mathrm{Dirac}}(\Omega,\mathbf{q})} = \frac{1}{\frac{|\mathbf{q}|}{2\pi\alpha v_x} + F_1\Pi(\Omega,\mathbf{q}) + F_2\Pi_{\mathrm{Dirac}}(\Omega,\mathbf{q})}, \tag{77}$$

where

$$\Pi(\Omega,\mathbf{q}) = \frac{1}{v_x d_y^{\frac{1}{3}}}\left[\frac{c_1 v_x^2 q_x^2}{\left(\Omega^2+v_x^2q_x^2+\frac{c_3^6}{c_2^6}d_y^2q_y^6\right)^{\frac{5}{6}}}+\frac{c_3 d_y^{\frac{2}{3}}q_y^2}{\left(\Omega^2+v_x^2q_x^2+\frac{c_3^6}{c_2^6}d_y^2q_y^6\right)^{\frac{1}{6}}}\right], \quad (78)$$

$$\Pi_{\mathrm{Dirac}}(\Omega,\mathbf{q}) = \frac{1}{16v_xv_y}\frac{v_x^2q_x^2+v_y^2q_y^2}{\sqrt{\Omega^2+v_x^2q_x^2+v_y^2q_y^2}}, \quad (79)$$

$$F_1 = e^{-\frac{v_y\Lambda}{d_y\Lambda^3}} = e^{-\frac{v_y}{d_y\Lambda^2}}, \quad (80)$$

$$F_2 = e^{-\frac{d_y\Lambda^3}{v_y\Lambda}} = e^{-\frac{d_y\Lambda^2}{v_y}}. \quad (81)$$

The fermion self-energy is given by

$$\Sigma(\omega,k) = \int\frac{d\Omega}{2\pi}\int'\frac{d^2\mathbf{q}}{(2\pi)^2}G_0^{new}\left(\omega+\Omega,\mathbf{k}+\mathbf{q}\right)V^\star(\Omega,\mathbf{q}). \quad (82)$$

Substituting the propagator of fermion, we get

$$\Sigma(\omega,\mathbf{k}) = \int\frac{d\Omega}{2\pi}\int'\frac{d^2\mathbf{q}}{(2\pi)^2}\frac{i\left(\omega+\Omega\right)+v_x\left(k_x+q_x\right)\sigma_1+\left[v_y\left(k_y+q_y\right)+d_y\left(k_y+q_y\right)^3\right]\sigma_2}{\left(\omega+\Omega\right)^2+v_x^2\left(k_x+q_x\right)^2+\left[v_y\left(k_y+q_y\right)+d_y\left(k_y+q_y\right)^3\right]^2}V^\star(\Omega,\mathbf{q}). \quad (83)$$

Expanding to leading order of $\omega$, $k_x$ and $k_y$, we get

$$\Sigma(\omega,\mathbf{k}) = -i\omega\Sigma_0+v_xk_x\sigma_1\Sigma_1+v_yk_y\sigma_2\Sigma_2^a+d_yk_y^3\sigma_2\Sigma_2^b \quad (84)$$

where

$$\Sigma_0 = \int\frac{d\Omega}{2\pi}\int'\frac{d^2\mathbf{q}}{(2\pi)^2}\frac{\Omega^2-\left(v_x^2q_x^2+v_y^2q_y^2+2v_yd_yq_y^4+d_y^2q_y^6\right)}{\left(\Omega^2+v_x^2q_x^2+v_y^2q_y^2+2v_yd_yq_y^4+d_y^2q_y^6\right)^2}V^\star(\Omega,\mathbf{q}), \quad (85)$$

$$\Sigma_1 = \int\frac{d\Omega}{2\pi}\int'\frac{d^2\mathbf{q}}{(2\pi)^2}\frac{\Omega^2-v_x^2q_x^2+v_y^2q_y^2+2v_yd_yq_y^4+d_y^2q_y^6}{\left(\Omega^2+v_x^2q_x^2+v_y^2q_y^2+2v_yd_yq_y^4+d_y^2q_y^6\right)^2}V^\star(\Omega,\mathbf{q}), \quad (86)$$

$$\Sigma_2^a = \int\frac{d\Omega}{2\pi}\int'\frac{d^2\mathbf{q}}{(2\pi)^2}\left\{\frac{1+3\frac{d_y}{v_y}q_y^2}{\Omega^2+v_x^2q_x^2+v_y^2q_y^2+2v_yd_yq_y^4+d_y^2q_y^6}\right.$$
$$\left.-\frac{2v_y^2q_y^2+10v_yd_yq_y^4+14d_y^2q_y^6+6\frac{d_y^3}{v_y}q_y^8}{\left(\Omega^2+v_x^2q_x^2+v_y^2q_y^2+2v_yd_yq_y^4+d_y^2q_y^6\right)^2}\right\}V^\star(\Omega,\mathbf{q}), \quad (87)$$

$$\Sigma_2^b = \int\frac{d\Omega}{2\pi}\int'\frac{d^2\mathbf{q}}{(2\pi)^2}\left\{\frac{1}{\Omega^2+v_x^2q_x^2+v_y^2q_y^2+2v_yd_yq_y^4+d_y^2q_y^6}\right.$$
$$-\frac{\frac{v_y^3}{d_y}+29v_y^2q_y^2+103v_yd_yq_y^4+83d_y^2q_y^6}{\left(\Omega^2+v_x^2q_x^2+v_y^2q_y^2+2v_yd_yq_y^4+d_y^2q_y^6\right)^2}$$
$$+\frac{8\frac{v_y^5}{d_y}q_y^2+112v_y^4q_y^4+512v_y^3d_yq_y^6+1008v_y^2d_y^2q_y^8+888v_yd_y^3q_y^{10}+288d_y^4q_y^{12}}{\left(\Omega^2+v_x^2q_x^2+v_y^2q_y^2+2v_yd_yq_y^4+d_y^2q_y^6\right)^3}$$
$$-\frac{1}{\left(\Omega^2+v_x^2q_x^2+v_y^2q_y^2+2v_yd_yq_y^4+d_y^2q_y^6\right)^4}\left[8\frac{v_y^7}{d_y}q_y^4+104v_y^6q_y^6+552v_y^5d_yq_y^8+1544v_y^4d_y^2q_y^{10}\right.$$
$$\left.\left.+2456v_y^3d_y^3q_y^{12}+2232v_y^2d_y^4q_y^{14}+1080v_yd_y^5q_y^{16}+216d_y^6q_y^{18}\right]\right\}V^\star(\Omega,\mathbf{q}). \quad (88)$$

We employ the RG scheme

$$-\infty<\Omega<+\infty, \quad (89)$$

$$b\Lambda<|\mathbf{q}|<\Lambda, \quad (90)$$

where $b = e^{-\ell}$ with $\ell$ being the RG running parameter. Carrying out tedious calculation, we obtain

$$\Sigma_0 = C_0^\star \ell, \quad (91)$$
$$\Sigma_1 = C_1^\star \ell, \quad (92)$$
$$\Sigma_2^a = C_2^{a\star} \ell, \quad (93)$$
$$\Sigma_2^b = C_2^{b\star} \ell, \quad (94)$$

where $C_1$, $C_2^a$, and $C_2^b$ are given by

$$C_0^\star = \frac{1}{8\pi^3}\int_{-\infty}^{+\infty} dx \int_0^{2\pi} d\varphi \frac{x^2 - \left(\cos^2(\varphi) + \delta^2\sin^2(\varphi) + 2\delta\beta\sin^4(\varphi) + \beta^2\sin^6(\varphi)\right)}{\left(x^2 + \cos^2(\varphi) + \delta^2\sin^2(\varphi) + 2\delta\beta\sin^4(\varphi) + \beta^2\sin^6(\varphi)\right)^2}\mathcal{G}(x,\varphi), \quad (95)$$

$$C_1^\star = \frac{1}{8\pi^3}\int_{-\infty}^{+\infty} dx \int_0^{2\pi} d\varphi \frac{x^2 - \cos^2(\varphi) + \delta^2\sin^2(\varphi) + 2\delta\beta\sin^4(\varphi) + \beta^2\sin^6(\varphi)}{\left(x^2 + \cos^2(\varphi) + \delta^2\sin^2(\varphi) + 2\delta\beta\sin^4(\varphi) + \beta^2\sin^6(\varphi)\right)^2}\mathcal{G}(x,\varphi), \quad (96)$$

$$\begin{aligned} C_2^{a\star} = {} & \frac{1}{8\pi^3}\int_{-\infty}^{+\infty} dx \int_0^{2\pi} d\varphi \Bigg\{ \frac{1 + 3\frac{1}{\delta}\beta\sin^2(\varphi)}{x^2 + \cos^2(\varphi) + \delta^2\sin^2(\varphi) + 2\delta\beta\sin^4(\varphi) + \beta^2\sin^6(\varphi)} \\ & - \frac{2\delta^2\sin^2(\varphi) + 10\delta\beta\sin^4(\varphi) + 14\beta^2\sin^6(\varphi) + 6\frac{1}{\delta}\beta^3\sin^8(\varphi)}{\left(x^2 + \cos^2(\varphi) + \delta^2\sin^2(\varphi) + 2\delta\beta\sin^4(\varphi) + \beta^2\sin^6(\varphi)\right)^2} \Bigg\} \mathcal{G}(x,\varphi), \end{aligned} \quad (97)$$

$$\begin{aligned} C_2^{b\star} = {} & \frac{1}{8\pi^3}\int_{-\infty}^{+\infty} dx \int_0^{2\pi} d\varphi \Bigg\{ \frac{1}{x^2 + \cos^2(\varphi) + \delta^2\sin^2(\varphi) + 2\delta\beta\sin^4(\varphi) + \beta^2\sin^6(\varphi)} \\ & - \frac{\delta^3\frac{1}{\beta} + 29\delta^2\sin^2(\varphi) + 103\delta\beta\sin^4(\varphi) + 83\beta^2\sin^6(\varphi)}{\left(x^2 + \cos^2(\varphi) + \delta^2\sin^2(\varphi) + 2\delta\beta\sin^4(\varphi) + \beta^2\sin^6(\varphi)\right)^2} \\ & + \frac{1}{\left(x^2 + \cos^2(\varphi) + \delta^2\sin^2(\varphi) + 2\delta\beta\sin^4(\varphi) + \beta^2\sin^6(\varphi)\right)^3}\Big[8\delta^5\frac{1}{\beta}\sin^2(\varphi) + 112\delta^4\sin^4(\varphi) + 512\delta^3\beta\sin^6(\varphi) \\ & + 1008\delta^2\beta^2\sin^8(\varphi) + 888\delta\beta^3\sin^{10}(\varphi) + 288\beta^4\sin^{12}(\varphi)\Big] \\ & - \frac{1}{\left(x^2 + \cos^2(\varphi) + \delta^2\sin^2(\varphi) + 2\delta\beta\sin^4(\varphi) + \beta^2\sin^6(\varphi)\right)^4}\Big[8\delta^7\frac{1}{\beta}\sin^4(\varphi) + 104\delta^6\sin^6(\varphi) + 552\delta^5\beta\sin^8(\varphi) \\ & + 1544\delta^4\beta^2\sin^{10}(\varphi) + 2456\delta^3\beta^3\sin^{12}(\varphi) + 2232\delta^2\beta^4\sin^{14}(\varphi) + 1080\delta\beta^5\sin^{16}(\varphi) \\ & + 216\beta^6\sin^{18}(\varphi)\Big]\Bigg\}\mathcal{G}(x,\varphi), \end{aligned} \quad (98)$$

with

$$\begin{aligned} \mathcal{G}^{-1}(x,\varphi) = {} & \frac{1}{2\pi\alpha} + e^{-\frac{v_y}{d_y\Lambda^2}}\left[\frac{c_1\beta^{-\frac{1}{3}}\cos^2(\varphi)}{\left(x^2 + \cos^2(\varphi) + \frac{c_3^6}{c_2^6}\beta^2\sin^6(\varphi)\right)^{\frac{5}{6}}} + \frac{c_3\beta^{\frac{1}{3}}\sin^2(\varphi)}{\left(x^2 + \cos^2(\varphi) + \frac{c_3^6}{c_2^6}\beta^2\sin^6(\varphi)\right)^{\frac{1}{6}}}\right] \\ & + e^{-\frac{d_y\Lambda^2}{v_y}}\frac{1}{16\delta}\frac{\cos^2(\varphi) + \delta^2\sin^2(\varphi)}{\sqrt{x^2 + \cos^2(\varphi) + \delta^2\sin^2(\varphi)}}. \end{aligned} \quad (99)$$

## B. Derivation of the RG equations

The action of free fermion is

$$S_\psi = \int \frac{d\omega}{2\pi}\frac{dk_x}{2\pi}\frac{dk_y}{2\pi}\psi^\dagger(\omega,\mathbf{k})\left(-i\omega + v_x k_x\sigma_1 + \left(v_y k_y + d_y k_y^3\right)\sigma_2\right)\psi(\omega,\mathbf{k}). \quad (100)$$

Consider the correction of self-energy of fermions, the action becomes

$$\begin{aligned} S_\psi &= \int \frac{d\omega}{2\pi}\frac{dk_x}{2\pi}\frac{dk_y}{2\pi}\psi^\dagger(\omega,\mathbf{k})\left(-i\omega + v_x k_x\sigma_1 + \left(v_y k_y + d_y k_y^3\right)\sigma_2 + \Sigma(\omega,\mathbf{k})\right)\psi(\omega,\mathbf{k}) \\ &= \int \frac{d\omega}{2\pi}\frac{dk_x}{2\pi}\frac{dk_y}{2\pi}\psi^\dagger(\omega,\mathbf{k})\left[-i\omega e^{C_0^\star\ell} + v_x k_x\sigma_1 e^{C_1^\star\ell} + \left(v_y k_y e^{C_2^{a\star}\ell} + d_y k_y^3 e^{C_2^{b\star}\ell}\right)\sigma_2\right]\psi(\omega,\mathbf{k}). \end{aligned} \quad (101)$$

Employing the transformations

$$
\begin{aligned}
k_x &= k'_x e^{-\ell}, & (102)\\
k_y &= k'_y e^{-\ell}, & (103)\\
\omega &= \omega' e^{-\ell}, & (104)\\
\psi &= \psi' e^{\left(2-\frac{C_0^\star}{2}\right)\ell}, & (105)\\
v_x &= v'_x e^{-(C_1^\star - C_0^\star)\ell}, & (106)\\
v_y &= v'_y e^{-(C_2^{a\star} - C_0^\star)\ell}, & (107)\\
d_y &= d'_y e^{\left(2-C_2^{b\star}+C_0^\star\right)\ell}, & (108)
\end{aligned}
$$

the action becomes

$$S_{\psi'} = \int \frac{d\omega'}{2\pi}\frac{dk'_x}{2\pi}\frac{dk'_y}{2\pi}\psi'^\dagger(\omega',\mathbf{k}')\left(-i\omega' + v'_x k'_x\sigma_1 + \left(v'_y k'_y + d'_y k'^3_y\right)\sigma_2\right)\psi'(\omega',\mathbf{k}'), \tag{109}$$

which recovers original form of the fermion action.

From Eqs. (106)-(108), we can get the RG equations for $v_x$, $v_y$, and $d_y$ as following

$$
\begin{aligned}
\frac{dv_x}{d\ell} &= \left(C_1^\star - C_0^\star\right)v_x, & (110)\\
\frac{dv_y}{d\ell} &= \left(C_2^{a\star} - C_0^\star\right)v_y, & (111)\\
\frac{dd_y}{d\ell} &= \left(-2 + C_2^{b\star} - C_0^\star\right)d_y. & (112)
\end{aligned}
$$

The RG equations for $\alpha$, $\beta$, and $\gamma$ can be written as

$$
\begin{aligned}
\frac{d\alpha}{d\ell} &= \left(-C_1^\star + C_0^\star\right)\alpha, & (113)\\
\frac{d\beta}{d\ell} &= \left(-2 - C_1^\star + C_2^{b\star}\right)\beta, & (114)\\
\frac{d\delta}{d\ell} &= \left(C_2^{a\star} - C_1^\star\right)\delta. & (115)
\end{aligned}
$$

## V. DYSON-SCHWINGER GAP EQUATION

### A. Derivation of the generation Dyson Schwinger gap equation

The free propagator of fermions with linear-cubic dispersion is given by

$$G_0(\omega,\mathbf{k}) = \frac{1}{-i\omega + v_x k_x\sigma_1 + d_y k_y^3\sigma_2}. \tag{116}$$

Including the renormalization of dispersion, the full fermion propagator can be written as

$$G_F(\omega,\mathbf{k}) = \frac{1}{-iA_0(\omega,k_x,k_y)\omega + A_1(\omega,k_x,k_y)v_x k_x\sigma_1 + A_2(\omega,k_x,k_y)d_y k_y^3\sigma_2. + \Delta(\omega,k_x,k_y)\sigma_3}, \tag{117}$$

where $A_{0,1,2}(\omega,k_x,k_y)$ represent the renormalized functions, and $\Delta(\omega,k_x,k_y)$ represent the dynamically generated excitonic gap. The full and free fermion propagators are connected by the following DS equation

$$G_F^{-1}(\varepsilon,\mathbf{p}) = G_0^{-1}(\varepsilon,\mathbf{p}) + \Sigma(\varepsilon,\mathbf{p}), \tag{118}$$

where the self-energy of fermion can be written as

$$\Sigma_{\varepsilon,\mathbf{p}} = \int\frac{d\omega}{2\pi}\frac{d^2\mathbf{k}}{(2\pi)^2}\Gamma(\varepsilon,\mathbf{p};\omega,\mathbf{k})G_F(\omega,\mathbf{k})V(\varepsilon-\omega,|\mathbf{p}-\mathbf{k}|), \tag{119}$$

where $\Gamma(\varepsilon, \mathbf{p}; \omega, \mathbf{k})$ is the vertex function, and $V(\varepsilon - \omega, |\mathbf{p} - \mathbf{k}|)$ is the dressed Coulomb interaction.

Tt is easy to obtain

$$A_0(\varepsilon, p_x, p_y) = 1 + \frac{1}{\varepsilon}\int_0^{+\infty}\frac{d\omega}{2\pi}\int\frac{d^2\mathbf{k}}{(2\pi)^2}\Gamma(\varepsilon, \mathbf{p}; \omega, \mathbf{k})\frac{A_0(\omega, k_x, k_y)\omega}{F(\omega, k_x, k_y)}\left[V(\varepsilon + \omega, |\mathbf{p} - \mathbf{k}|) - V(\varepsilon - \omega, |\mathbf{p} - \mathbf{k}|)\right], \quad (120)$$

$$A_1(\varepsilon, p_x, p_y) = 1 + \frac{1}{p_x}\int_0^{+\infty}\frac{d\omega}{2\pi}\int\frac{d^2\mathbf{k}}{(2\pi)^2}\Gamma(\varepsilon, \mathbf{p}; \omega, \mathbf{k})\frac{A_1(\omega, k_x, k_y)k_x}{F(\omega, k_x, k_y)}\left[V(\varepsilon + \omega, |\mathbf{p} - \mathbf{k}|) + V(\varepsilon - \omega, |\mathbf{p} - \mathbf{k}|)\right], \quad (121)$$

$$A_2(\varepsilon, p_x, p_y) = 1 + \frac{1}{p_y^3}\int_0^{+\infty}\frac{d\omega}{2\pi}\int\frac{d^2\mathbf{k}}{(2\pi)^2}\Gamma(\varepsilon, \mathbf{p}; \omega, \mathbf{k})\frac{A_2(\omega, k_x, k_y)k_y^3}{F(\omega, k_x, k_y)}\left[V(\varepsilon + \omega, |\mathbf{p} - \mathbf{k}|) + V(\varepsilon - \omega, |\mathbf{p} - \mathbf{k}|)\right], \quad (122)$$

$$\Delta(\varepsilon, p_x, p_y) = \int\frac{d\omega}{2\pi}\frac{d^2\mathbf{k}}{(2\pi)^2}\Gamma(\varepsilon, \mathbf{p}; \omega, \mathbf{k})\frac{\Delta(\omega, k_x, k_y)}{F(\omega, k_x, k_y)}V(\varepsilon - \omega, |\mathbf{p} - \mathbf{k}|), \quad (123)$$

where

$$F(\omega, k_x, k_y) = A_0(\omega, k_x, k_y)\omega A_0^2(\omega, k_x, k_y)\omega + A_1^2(\omega, k_x, k_y)v_x^2k_x^2 + A_2^2(\omega, k_x, k_y)d_y^2k_y^6 + \Delta^2(\omega, k_x, k_y). \quad (124)$$

The relations

$$A_{0,1,2}(\varepsilon, p_x, p_y) = A_{0,1,2}(-\varepsilon, p_x, p_y), \quad (125)$$

$$m(\varepsilon, p_x, p_y) = m(-\varepsilon, p_x, p_y), \quad (126)$$

which have been determined by particle-hole symmetry, have been used.

The dressed Coulomb interaction is given by

$$V(\Omega, \mathbf{q}) = \frac{1}{\frac{|\mathbf{q}|}{2\pi\alpha v_x} + \Pi(\Omega, \mathbf{q})}. \quad (127)$$

The polarization can be calculated self-consistently through

$$\Pi(\Omega, \mathbf{q}) = -N\int\frac{d\omega}{2\pi}\int\frac{d^2\mathbf{k}}{(2\pi)^2}\mathrm{Tr}\left[\Gamma(\omega, \mathbf{k}; \omega + \Omega, \mathbf{k} + \mathbf{q})G_F(\omega, \mathbf{k})G_F(\omega + \Omega, \mathbf{k} + \mathbf{q})\right]. \quad (128)$$

In principle, the Dyson-Schwinger equation for full vertex function can be written down. However, this will lead to infinite coupled equations. In order to solve the Dyson-schwinger equations, we have to truncate the equations by employ some ansatz for the vertex correction [1–4]. The ansatz has a form which satisfies Ward identity. We can take the following ansatz

$$\Gamma(\varepsilon, \mathbf{p}; \omega, \mathbf{k}) = \frac{A_0(\varepsilon, p_x, p_y) + A_0(\omega, k_x, k_y)}{2}, \quad (129)$$

which has been utilized in some related questions.

Solving the Eqs. (120)-(123), (127), (128) and (129) numerically, we can obtain the renormalized functions $A_{0,1,2}(\varepsilon, p_x, p_y)$ and the dynamically generated gap $\Delta(\varepsilon, p_x, p_y)$. However, due to the explicit breaking of Lorentz invariance by Coulomb interaction and anisotropy of the fermion dispersion, $A_{0,1,2}(\varepsilon, p_x, p_y)$ and $\Delta(\varepsilon, p_x, p_y)$ depend on three variable separately. Therefore, numerical calculation the above equations is very challenge. In the following, we simply the equations by employing approximations which are widely utilized.

## B. Gap equation under approximations

### 1. Lowest order approximation

In the lowest order approximation, taking $A_{0,1,2}(\varepsilon, p_x, p_y) \equiv 1$, and vertex function $\Gamma \equiv 1$ to satisfy Ward indenisty, and neglecting the the correction to Coulomb interaction from the polarization function, the gap equation can be written as

$$\Delta(\varepsilon, p_x, p_y) = 2\int_0^{+\infty}\frac{d\omega}{2\pi}\int\frac{d^2\mathbf{k}}{(2\pi)^2}\frac{\Delta(k_x, k_y)}{\omega^2 + v_x^2k_x^2 + d_y^2k_y^6 + \Delta^2(\omega, k_x, k_y)}V_0(\mathbf{p} - \mathbf{k}), \quad (130)$$

In this case, we can find that $\Delta$ actually is independent of energy, thus the gap equation can be further written as

$$\begin{aligned}\Delta(p_x,p_y) &= 2\int_0^{+\infty}\frac{d\omega}{2\pi}\int\frac{d^2\mathbf{k}}{(2\pi)^2}\frac{\Delta(k_x,k_y)}{\omega^2+v_x^2k_x^2+d_y^2k_y^6+\Delta^2(k_x,k_y)}\frac{2\pi\alpha v_x}{|\mathbf{p}-\mathbf{k}|}\\ &= \pi\alpha v_x\int\frac{d^2\mathbf{k}}{(2\pi)^2}\frac{\Delta(k_x,k_y)}{\sqrt{v_x^2k_x^2+d_y^2k_y^6+\Delta^2(k_x,k_y)}}\frac{1}{|\mathbf{p}-\mathbf{k}|} \end{aligned}\tag{131}$$

The gap equaiton can be further written as

$$\Delta(p_x,p_y) = \pi\alpha v_x\frac{1}{4\pi^2}\int_{-\Lambda_x}^{\Lambda_x}dk_x\int_{-\Lambda_y}^{\Lambda_y}dk_y\frac{\Delta(k_x,k_y)}{\sqrt{v_x^2k_x^2+d_y^2k_y^6+\Delta^2(k_x,k_y)}}\frac{1}{\sqrt{(p_x-k_x)^2+(p_y-k_y)^2}}.\tag{132}$$

Let

$$P_x = \frac{p_x}{\Lambda_x},\tag{133}$$

$$P_y = \frac{p_y}{\Lambda_y},\tag{134}$$

$$K_x = \frac{k_x}{\Lambda_x},\tag{135}$$

$$K_y = \frac{k_y}{\Lambda_y},\tag{136}$$

$$\Delta'(P_x,P_y) = \frac{\Delta(P_x,P_y)}{v_x\Lambda_x},\tag{137}$$

and take

$$\Lambda_x=\Lambda_y=\Lambda,\tag{138}$$

we can get

$$\Delta'(P_x,P_y) = \alpha\frac{1}{4\pi}\int_{-1}^{1}dK_x\int_{-1}^{1}dK_y\frac{\Delta'(K_x,K_y)}{\sqrt{K_x^2+\beta^2K_y^6+\Delta'^2(K_x,K_y)}}\frac{1}{\sqrt{(P_x-K_x)^2+(P_y-K_y)^2}},\tag{139}$$

where

$$\beta = \frac{d_y\Lambda^2}{v_x}.\tag{140}$$

### C. Dressed Coulomb interaction

The polarization to lowest order is given by Eq. (32). Considering the correction from polarization, the dressed long-range Coulomb interaction can be written as

$$V(\Omega,\mathbf{q}) = \frac{1}{V_0^{-1}(|\mathbf{q}|)+\Pi(\Omega,\mathbf{q})} = \frac{1}{\frac{|\mathbf{q}|}{2\pi\alpha v_x}+\frac{1}{v_xd_y^{\frac{1}{3}}}\left[\frac{c_1v_x^2q_x^2}{\left(\Omega^2+v_x^2q_x^2+\frac{c_3^6}{c_2^6}d_y^2q_y^6\right)^{\frac{5}{6}}}+\frac{c_3d_y^{\frac{2}{3}}q_y^2}{\left(\Omega^2+v_x^2q_x^2+\frac{c_3^6}{c_2^6}d_y^2q_y^6\right)^{\frac{1}{6}}}\right]}.\tag{141}$$

Accordingly, the gap equation can be written as

$$\Delta(\varepsilon,p_x,p_y) = \int_0^{+\infty}\frac{d\omega}{2\pi}\int\frac{d^2\mathbf{k}}{(2\pi)^2}\frac{\Delta(k_x,k_y)}{\omega^2+v_x^2k_x^2+d_y^2k_y^6+\Delta^2(\omega,k_x,k_y)}\left[V(\varepsilon-\omega,\mathbf{p}-\mathbf{k})+V(\varepsilon+\omega,\mathbf{p}-\mathbf{k})\right].\tag{142}$$

The paritcle-hole symmetry

$$\Delta(\varepsilon,p_x,p_y)=\Delta(-\varepsilon,p_x,p_y),\tag{143}$$

has been used.

Employing the instantaneous approximation [5–8],

$$V(\Omega,\mathbf{q}) \rightarrow V(0,\mathbf{q}), \tag{144}$$

we get

$$\begin{aligned}\Delta(p_x,p_y) &= 2\int_0^{+\infty}\frac{d\omega}{2\pi}\int\frac{d^2\mathbf{k}}{(2\pi)^2}\frac{\Delta(k_x,k_y)}{\omega^2+v_x^2k_x^2+d_y^2k_y^6+\Delta^2(k_x,k_y)}V(0,\mathbf{p}-\mathbf{k})\\ &= \frac{1}{2}\int\frac{d^2\mathbf{k}}{(2\pi)^2}\frac{\Delta(k_x,k_y)}{\sqrt{v_x^2k_x^2+d_y^2k_y^6+\Delta^2(k_x,k_y)}}V(0,\mathbf{p}-\mathbf{k}).\end{aligned} \tag{145}$$

The gap equation can be further written as

$$\begin{aligned}\Delta'(P_x,P_y) &= \frac{1}{8\pi^2}\int_{-1}^{1}dK_x\int_{-1}^{1}dK_y\frac{\Delta'(K_x,K_y)}{\sqrt{K_x^2+\beta^2K_y^6+\Delta'^2(K_x,K_y)}}\left[\frac{\sqrt{\left(P_x-K_x\right)^2+\left(P_y-K_y\right)^2}}{2\pi\alpha}\right.\\ &\left.+\left\{\frac{c_1\left(P_x-K_x\right)^2}{\beta^{\frac{1}{3}}\left[\left(P_x-K_x\right)^2+\frac{c_3^6}{c_2^6}\beta^2\left(P_y-K_y\right)^6\right]^{\frac{5}{6}}}+\frac{c_3\beta^{\frac{1}{3}}\left(P_y-K_y\right)^2}{\left[\left(P_x-K_x\right)^2+\frac{c_3^6}{c_2^6}\beta^2\left(P_y-K_y\right)^6\right]^{\frac{1}{6}}}\right\}\right]^{-1}.\end{aligned} \tag{146}$$

Eqs. (133)-(137) have been used.

## VI. OBSERVABLE QUANTITIES

### A. Density of states

Considering a constant excitonic gap $\Delta$, the retarded fermion propagator takes the form

$$G_{\Delta}^{\mathrm{ret}}(\omega,\mathbf{k}) = \frac{1}{-\omega+\mathcal{H}_{\mathbf{k}\Delta}-i\eta}, \tag{147}$$

where

$$H_{\mathbf{k}\Delta} = v_xk_x\sigma_1+d_yk_y^3\sigma_2+\Delta\sigma_3, \tag{148}$$

and $\eta$ is infinitesimal. The imaginary part of the fermion propagator is

$$\mathrm{Im}\left[G_{\Delta}^{\mathrm{ret}}(\omega,\mathbf{k})\right] = \pi\mathrm{sgn}(\omega)\left(\omega+\mathcal{H}_{\mathbf{k}\Delta}\right)\frac{1}{2E_{\mathbf{k}\Delta}}\left[\delta\left(\omega+E_{\mathbf{k}\Delta}\right)+\delta\left(\omega-E_{\mathbf{k}\Delta}\right)\right], \tag{149}$$

where

$$E_{\mathbf{k}\Delta} = \sqrt{v_x^2k_x^2+d_y^2k_y^6+\Delta^2}. \tag{150}$$

The spectral function is given by

$$A(\omega,\mathbf{k}) = \frac{1}{\pi}\mathrm{Tr}\left[\mathrm{Im}\left[G_{\Delta}^{\mathrm{ret}}(\omega,\mathbf{k})\right]\right] = \frac{|\omega|}{E_{\mathbf{k}\Delta}}\left[\delta\left(\omega+E_{\mathbf{k}\Delta}\right)+\delta\left(\omega-E_{\mathbf{k}\Delta}\right)\right]. \tag{151}$$

The density of states can be written as

$$\begin{aligned}\rho(\omega) &= \int\frac{d^2\mathbf{k}}{(2\pi)^2}A(\omega,\mathbf{k})\\ &= \frac{1}{\pi^2}\int_0^{+\infty}\int_0^{+\infty}dk_xdk_y\frac{|\omega|}{E_{\mathbf{k}\Delta}}\left[\delta\left(\omega+E_{\mathbf{k}\Delta}\right)+\delta\left(\omega-E_{\mathbf{k}\Delta}\right)\right].\end{aligned} \tag{152}$$

In the following, we employ the transformations

$$E = \sqrt{v_x^2 k_x^2 + d_y^2 k_y^6}, \tag{153}$$

$$\xi = \frac{d_y k_y^3}{v_x k_x}, \tag{154}$$

which are equivalent to

$$k_x = \frac{E}{v_x \sqrt{1+\xi^2}}, \tag{155}$$

$$k_y = \frac{\xi^{\frac{1}{3}} E^{\frac{1}{3}}}{d_y^{\frac{1}{3}} \left(1+\xi^2\right)^{\frac{1}{6}}}, \tag{156}$$

The measures of the integrations satisfy the relation

$$dk_x dk_y = \left\| \begin{array}{cc} \frac{\partial k_x}{\partial E} & \frac{\partial k_x}{\partial \xi} \\ \frac{\partial k_y}{\partial E} & \frac{\partial k_y}{\partial \xi} \end{array} \right\| dE d\xi = \left| \frac{\partial k_x}{\partial E}\frac{\partial k_y}{\partial \xi} - \frac{\partial k_y}{\partial E}\frac{\partial k_x}{\partial \xi} \right| dE d\xi = \frac{E^{\frac{1}{3}}}{3 v_x d_y^{\frac{1}{3}} \xi^{\frac{2}{3}} \left(1+\delta^2\right)^{\frac{2}{3}}} dE d\xi. \tag{157}$$

Utilizing the Eqs. (153)-(157), we obtain

$$\rho(\omega) = \frac{\Gamma\left(\frac{7}{6}\right)}{\pi^{\frac{3}{2}}\Gamma\left(\frac{2}{3}\right)} \frac{1}{v_x d_y^{\frac{1}{3}}} \frac{|\omega|}{\left(\omega^2-\Delta^2\right)^{\frac{1}{3}}} \theta\left(|\omega|-\Delta\right), \tag{158}$$

where $\Gamma(x)$ is the Gamma function.

For $\Delta = 0$, we have

$$\rho(\omega) = \frac{\Gamma\left(\frac{7}{6}\right)}{\pi^{\frac{3}{2}}\Gamma\left(\frac{2}{3}\right)} \frac{1}{v_x d_y^{\frac{1}{3}}} |\omega|^{\frac{1}{3}}. \tag{159}$$

### B. Specific heat

The propagator of fermions in Matsubara formalism can be written as

$$G_\Delta(\omega_n, \mathbf{k}) = \frac{1}{-i\omega_n + v_x k_x \sigma_1 + d_y k_y^3 \sigma_2 + \Delta\sigma_3} = \frac{i\omega_n + v_x k_x \sigma_1 + d_y k_y^3 \sigma_2 + \Delta\sigma_3}{\omega_n^2 + E_{\mathbf{k},\Delta}^2}, \tag{160}$$

where $\omega_n = (2n+1)\pi T$ with $n$ being integers and $T$ the temperature.

The free energy of the fermion is

$$F_f(T) = -2T \sum_{\omega_n} \int \frac{d^2\mathbf{k}}{(2\pi)^2} \ln\left[\left(\omega_n^2 + E_{\mathbf{k},\Delta}^2\right)^{\frac{1}{2}}\right]. \tag{161}$$

Carrying out the frequency summation, we obtain

$$F_f(T) = -2\int \frac{d^2\mathbf{k}}{(2\pi)^2}\left[E_{\mathbf{k}\Delta} + 2T\ln\left(1+e^{-\frac{E_{\mathbf{k}\Delta}}{T}}\right)\right], \tag{162}$$

which is clearly divergent. In order to get a finite free energy, we redefine $F_f(T) - F_f(0)$ as $F_f(T)$, and then get

$$\begin{aligned} F_f(T) &= -4T\int \frac{d^2\mathbf{k}}{(2\pi)^2}\ln\left(1+e^{-\frac{E_{\mathbf{k}\Delta}}{T}}\right) \\ &= -\frac{4T}{\pi^2}\int_0^{+\infty}\int_0^{+\infty} dk_x dk_y \ln\left(1+e^{-\frac{\sqrt{v_x^2k_x^2+d_y^2k_y^6+\Delta^2}}{T}}\right). \end{aligned} \tag{163}$$

Using the transformations Eqs. (153)-(157), we arrive

$$\begin{aligned} F_f(T) &= -\frac{4T}{3\pi^2 v_x d_y^{\frac{1}{3}}}\int_0^{+\infty} dE E^{\frac{1}{3}} \ln\left(1+e^{-\frac{\sqrt{E^2+\Delta^2}}{T}}\right)\int_0^{+\infty} d\xi \frac{1}{\xi^{\frac{2}{3}}\left(1+\xi^2\right)^{\frac{2}{3}}} \\ &= -\frac{4\Gamma\left(\frac{7}{6}\right)T}{\pi^{\frac{3}{2}}\Gamma\left(\frac{2}{3}\right)v_x d_y^{\frac{1}{3}}}\int_0^{+\infty} dE E^{\frac{1}{3}} \ln\left(1+e^{-\frac{\sqrt{E^2+\Delta^2}}{T}}\right). \end{aligned} \quad (164)$$

The specific heat is defined as

$$C_v(T) = -T\frac{\partial^2 F_f(T)}{\partial T^2}. \quad (165)$$

Then we can get

$$C_v(T) = \frac{4\Gamma\left(\frac{7}{6}\right)T}{\pi^{\frac{3}{2}}\Gamma\left(\frac{2}{3}\right)v_x d_y^{\frac{1}{3}}}T^{\frac{1}{3}}\int_0^{+\infty} dx x^{\frac{1}{3}}\frac{e^{\sqrt{x^2+\left(\frac{\Delta}{T}\right)^2}}}{\left[1+e^{\sqrt{x^2+\left(\frac{\Delta}{T}\right)^2}}\right]^2}\left[x^2+\left(\frac{\Delta}{T}\right)^2\right]. \quad (166)$$

For $\Delta=0$, we have

$$\begin{aligned} C_v(T) &= \frac{4\Gamma\left(\frac{7}{6}\right)T}{\pi^{\frac{3}{2}}\Gamma\left(\frac{2}{3}\right)v_x d_y^{\frac{1}{3}}}T^{\frac{1}{3}}\int_0^{+\infty} dx x^{\frac{7}{3}}\frac{e^x}{\left(1+e^x\right)^2} \\ &= \frac{28\left(4-2^{\frac{2}{3}}\right)\zeta\left(\frac{7}{3}\right)\Gamma\left(\frac{4}{3}\right)\Gamma\left(\frac{7}{6}\right)}{9\pi^{\frac{3}{2}}\Gamma\left(\frac{2}{3}\right)}\frac{1}{v_x d_y^{\frac{1}{3}}}T^{\frac{4}{3}}, \end{aligned} \quad (167)$$

where $\zeta(x)$ is the Riemann zeta function.

For finite $\Delta$, in the limit $T \ll \Delta$, $C_v$ can be approximately by

$$\begin{aligned} C_v(T) &\approx \frac{4\Gamma\left(\frac{7}{6}\right)}{\pi^{\frac{3}{2}}\Gamma\left(\frac{2}{3}\right)v_x d_y^{\frac{1}{3}}}T^{\frac{4}{3}}\left\{\int_0^{\frac{\Delta}{T}} dx x^{\frac{1}{3}}\frac{e^{\frac{\Delta}{T}}}{\left[1+e^{\frac{\Delta}{T}}\right]^2}\left[x^2+\left(\frac{\Delta}{T}\right)^2\right]+\int_{\frac{\Delta}{T}}^{+\infty} dx x^{\frac{1}{3}}\frac{e^x}{\left[1+e^x\right]^2}x^2\right\} \\ &\approx \frac{21\Gamma\left(\frac{7}{6}\right)}{5\pi^{\frac{3}{2}}\Gamma\left(\frac{2}{3}\right)}\frac{1}{v_x d_y^{\frac{1}{3}}}\frac{\Delta^{\frac{10}{3}}}{T^2}e^{-\frac{\Delta}{T}}. \end{aligned} \quad (168)$$

### C. Compressibility

Considering a finite chemical potential $\mu$, the propagator fermions in Matsubara formalism can be written as

$$\begin{aligned} G_\Delta(\omega_n,\mathbf{k}) &= \frac{1}{-\left(i\omega_n+\mu\right)+v_x k_x\sigma_1+d_y k_y^3 k_y\sigma_2+\Delta\sigma_3} \\ &= \frac{i\omega_n+\mu+v_x k_x\sigma_1+d_y k_y^3\sigma_2+\Delta\sigma_3}{\left(\omega_n-i\mu\right)^2+v_x^2k_x^2+d_y^2k_y^6+\Delta^2}. \end{aligned} \quad (169)$$

The free energy of the fermion is

$$F_f(T,\mu) = -2T\sum_{\omega_n}\int\frac{d^2\mathbf{k}}{(2\pi)^2}\ln\left[\left(\left(\omega_n-i\mu\right)^2+E_{\mathbf{k},\Delta}^2\right)^{\frac{1}{2}}\right]. \quad (170)$$

Performing the frequency summation and discarding the divergent term by redefining $F_f(T)-F_f(0)$ as $F_f(T)$, we get

$$\begin{aligned} F_f(T,\mu) &= -2T\sum_{\zeta=\pm1}\int\frac{d^2\mathbf{k}}{(2\pi)^2}\ln\left(1+e^{-\frac{E_k+\zeta\mu}{T}}\right) \\ &= -\frac{2T}{\pi^2}\sum_{\zeta=\pm1}\int_0^{+\infty}\int_0^{+\infty} dk_x dk_y \ln\left(1+e^{-\frac{\sqrt{v_x^2k_x^2+d_y^2k_y^6+\Delta^2}+\zeta\mu}{T}}\right). \end{aligned} \quad (171)$$

Using the transformations Eqs. (153)-(157), we obtain

$$F_f(T,\mu) = -\frac{2\Gamma\left(\frac{7}{6}\right)T}{\pi^{\frac{3}{2}}\Gamma\left(\frac{2}{3}\right)v_x d_y^{\frac{1}{3}}}\sum_{\zeta=\pm1}\int_0^{+\infty} dE E^{\frac{1}{3}}\ln\left(1+e^{-\frac{\sqrt{E^2+\Delta^2}+\zeta\mu}{T}}\right). \quad (172)$$

Using the formula

$$\kappa = -\frac{\partial^2 F_f(T,\mu)}{\partial\mu^2}, \quad (173)$$

we can get the compressibility

$$\kappa(T,\mu) = \frac{2\Gamma\left(\frac{7}{6}\right)}{\pi^{\frac{3}{2}}\Gamma\left(\frac{2}{3}\right)}\frac{1}{v_x d_y^{\frac{1}{3}}T}\sum_{\alpha=\pm1}\int_0^{+\infty} dE E^{\frac{1}{3}}\frac{e^{\frac{\sqrt{E^2+\Delta^2}+\alpha\mu}{T}}}{\left(1+e^{\frac{\sqrt{E^2+\Delta^2}+\alpha\mu}{T}}\right)^2}. \quad (174)$$

For $\mu = 0$, we have

$$\kappa(T) = \frac{4\Gamma\left(\frac{7}{6}\right)}{\pi^{\frac{3}{2}}\Gamma\left(\frac{2}{3}\right)}\frac{1}{v_x d_y^{\frac{1}{3}}}T^{\frac{1}{3}}\int_0^{+\infty} dx x^{\frac{1}{3}}\frac{e^{\sqrt{x^2+\left(\frac{\Delta}{T}\right)^2}}}{\left(1+e^{\sqrt{x^2+\left(\frac{\Delta}{T}\right)^2}}\right)^2}. \quad (175)$$

In the case $\Delta = 0$, we have

$$\begin{aligned}\kappa(T) &= \frac{4\Gamma\left(\frac{7}{6}\right)}{\pi^{\frac{3}{2}}\Gamma\left(\frac{2}{3}\right)}\frac{1}{v_x d_y^{\frac{1}{3}}}T^{\frac{1}{3}}\int_0^{+\infty} dx x^{\frac{1}{3}}\frac{e^x}{(1+e^x)^2} \\ &= \frac{4\left(1-2^{\frac{2}{3}}\right)\zeta\left(\frac{1}{3}\right)\Gamma\left(\frac{7}{6}\right)\Gamma\left(\frac{4}{3}\right)}{\pi^{\frac{3}{2}}\Gamma\left(\frac{2}{3}\right)v_x d_y^{\frac{1}{3}}}T^{\frac{1}{3}}. \quad (176)\end{aligned}$$

For finite $\Delta$, in the limit $T \ll \Delta$, the compressibility can be approximated as

$$\begin{aligned}\kappa(T) &\approx \frac{4\Gamma\left(\frac{7}{6}\right)}{\pi^{\frac{3}{2}}\Gamma\left(\frac{2}{3}\right)}\frac{1}{v_x d_y^{\frac{1}{3}}}T^{\frac{1}{3}}\left[\int_0^{\frac{\Delta}{T}} dx x^{\frac{1}{3}}\frac{e^{\frac{\Delta}{T}}}{\left(1+e^{\frac{\Delta}{T}}\right)^2}+\int_{\frac{\Delta}{T}}^{+\infty} dx x^{\frac{1}{3}}\frac{e^x}{(1+e^x)^2}\right] \\ &\approx \frac{3\Gamma\left(\frac{7}{6}\right)}{\pi^{\frac{3}{2}}\Gamma\left(\frac{2}{3}\right)}\frac{1}{v_x d_y^{\frac{1}{3}}}\frac{\Delta^{\frac{4}{3}}}{T}e^{-\frac{\Delta}{T}}. \quad (177)\end{aligned}$$

### D. Electric conductivity

The current-current correlation function is given by

$$\Pi_{ij}(i\Omega_m) = -e^2T\sum_{\omega_n}\int\frac{d^3\mathbf{k}}{(2\pi)^3}\mathrm{Tr}\left[\gamma_i(\mathbf{k})G_\Delta(i\omega_n,\mathbf{k})\gamma_j(\mathbf{k})G_\Delta(i(\omega_n+\Omega_m),\mathbf{k})\right], \quad (178)$$

where

$$\gamma_i = \frac{\partial\mathcal{H}_\Delta}{\partial k_i}, \quad (179)$$

with

$$\mathcal{H}_\Delta = v_x k_x\sigma_1 + d_y k_y^3\sigma_2 + \Delta\sigma_3. \quad (180)$$

It is easy to verify that

$$\gamma_x = v_x\sigma_1, \tag{181}$$
$$\gamma_y = 3d_y k_y^2\sigma_2. \tag{182}$$

Concretely, $\Pi_{xx}$ and $\Pi_{yy}$ are given by

$$\Pi_{xx}(i\Omega_m) = -v_x^2e^2T\sum_{\omega_n}\int\frac{d^2\mathbf{k}}{(2\pi)^2}\mathrm{Tr}\left[\sigma_1 G_\Delta(i\omega_n,\mathbf{k})\sigma_1 G_\Delta(i(\omega_n+\Omega_m),\mathbf{k})\right], \tag{183}$$
$$\Pi_{yy}(i\Omega_m) = -9d_y^2e^2T\sum_{\omega_n}\int\frac{d^2\mathbf{k}}{(2\pi)^2}k_y^4\mathrm{Tr}\left[\sigma_2 G_\Delta(i\omega_n,\mathbf{k})\sigma_2 G_\Delta(i(\omega_n+\Omega_m),\mathbf{k})\right]. \tag{184}$$

Using the standard frequency representation

$$G_\Delta\left(i\omega_n,\mathbf{k}\right) = -\int_{-\infty}^{+\infty}\frac{d\omega_1}{\pi}\frac{\mathrm{Im}\left[G_\Delta^{\mathrm{ret}}\left(\omega_1,\mathbf{k}\right)\right]}{i\omega_n-\omega_1}, \tag{185}$$

we have

$$\begin{aligned}\Pi_{xx}(i\Omega_m) &= -v_x^2e^2\int\frac{d^2\mathbf{k}}{(2\pi)^2}\int_{-\infty}^{+\infty}\frac{d\omega_1}{\pi}\int_{-\infty}^{+\infty}\frac{d\omega_2}{\pi}\mathrm{Tr}\left[\sigma_1\mathrm{Im}\left[G_\Delta^{\mathrm{ret}}\left(\omega_1,\mathbf{k}\right)\right]\sigma_1\mathrm{Im}\left[G_\Delta^{\mathrm{ret}}\left(\omega_2,\mathbf{k}\right)\right]\right]\\ &\quad\times T\sum_{\omega_n}\frac{1}{i\omega_n-\omega_1}\frac{1}{i\omega_n+i\Omega_m-\omega_2},\end{aligned} \tag{186}$$
$$\begin{aligned}\Pi_{yy}(i\Omega_m) &= -9d_y^2e^2\int\frac{d^2\mathbf{k}}{(2\pi)^2}k_y^4\int_{-\infty}^{+\infty}\frac{d\omega_1}{\pi}\int_{-\infty}^{+\infty}\frac{d\omega_2}{\pi}\mathrm{Tr}\left[\sigma_2\mathrm{Im}\left[G_\Delta^{\mathrm{ret}}\left(\omega_1,\mathbf{k}\right)\right]\sigma_2\mathrm{Im}\left[G_\Delta^{\mathrm{ret}}\left(\omega_2,\mathbf{k}\right)\right]\right]\\ &\quad\times T\sum_{\omega_n}\frac{1}{i\omega_n-\omega_1}\frac{1}{i\omega_n+i\Omega_m-\omega_2}.\end{aligned} \tag{187}$$

Performing the frequency summation, we arrive

$$\Pi_{xx}(i\Omega_m) = -v_x^2e^2\int\frac{d^2\mathbf{k}}{(2\pi)^2}\int_{-\infty}^{+\infty}\frac{d\omega_1}{\pi}\int_{-\infty}^{+\infty}\frac{d\omega_2}{\pi}\mathrm{Tr}\left[\sigma_1\mathrm{Im}\left[G_\Delta^{\mathrm{ret}}\left(\omega_1,\mathbf{k}\right)\right]\sigma_1\mathrm{Im}\left[G_\Delta^{\mathrm{ret}}\left(\omega_2,\mathbf{k}\right)\right]\right], \tag{188}$$
$$\times\frac{n_F\left(\omega_1\right)-n_F\left(\omega_2\right)}{\omega_1-\omega_2+i\Omega_m} \tag{189}$$
$$\begin{aligned}\Pi_{yy}(i\Omega_m) &= -9d_y^2e^2\int\frac{d^2\mathbf{k}}{(2\pi)^2}k_y^4\int_{-\infty}^{+\infty}\frac{d\omega_1}{\pi}\int_{-\infty}^{+\infty}\frac{d\omega_2}{\pi}\mathrm{Tr}\left[\sigma_2\mathrm{Im}\left[G_\Delta^{\mathrm{ret}}\left(\omega_1,\mathbf{k}\right)\right]\sigma_2\mathrm{Im}\left[G_\Delta^{\mathrm{ret}}\left(\omega_2,\mathbf{k}\right)\right]\right]\\ &\quad\times\frac{n_F\left(\omega_1\right)-n_F\left(\omega_2\right)}{\omega_1-\omega_2+i\Omega_m},\end{aligned} \tag{190}$$

where $n_F(x) = \frac{1}{e^{\frac{x}{T}}+1}$. Carrying out the analytical continuation $i\Omega_m \to \Omega + i\eta$, and using the formula

$$\frac{1}{x+i\eta} = \mathcal{P}\frac{1}{x} - i\pi\delta(x), \tag{191}$$

where $\mathcal{P}$ represents the principal value, we can get

$$\begin{aligned}\mathrm{Im}\left[\Pi_{xx}^{\mathrm{ret}}(\Omega,T)\right] &= v_x^2e^2\int\frac{d^2\mathbf{k}}{(2\pi)^2}\int_{-\infty}^{+\infty}\frac{d\omega_1}{\pi}\mathrm{Tr}\left[\sigma_1\mathrm{Im}\left[G_\Delta^{\mathrm{ret}}\left(\omega_1,\mathbf{k}\right)\right]\sigma_1\mathrm{Im}\left[G_\Delta^{\mathrm{ret}}\left(\omega_1+\Omega,\mathbf{k}\right)\right]\right]\\ &\quad\times\left[n_F\left(\omega_1\right)-n_F\left(\omega_1+\Omega\right)\right],\end{aligned} \tag{192}$$
$$\begin{aligned}\mathrm{Im}\left[\Pi_{yy}^{\mathrm{ret}}(\Omega,T)\right] &= 9d_y^2e^2\int\frac{d^2\mathbf{k}}{(2\pi)^2}k_y^4\int_{-\infty}^{+\infty}\frac{d\omega_1}{\pi}\mathrm{Tr}\left[\sigma_2\mathrm{Im}\left[G_\Delta^{\mathrm{ret}}\left(\omega_1,\mathbf{k}\right)\right]\sigma_2\mathrm{Im}\left[G_\Delta^{\mathrm{ret}}\left(\omega_1+\Omega,\mathbf{k}\right)\right]\right]\\ &\quad\times\left[n_F\left(\omega_1\right)-n_F\left(\omega_1+\Omega\right)\right].\end{aligned} \tag{193}$$

The conductivities are defined as

$$\sigma_{xx}(\Omega,T) = \frac{\mathrm{Im}\left[\Pi^{\mathrm{ret}}_{xx}(\Omega,T)\right]}{\Omega}, \tag{194}$$

$$\sigma_{yy}(\Omega,T) = \frac{\mathrm{Im}\left[\Pi^{\mathrm{ret}}_{yy}(\Omega,T)\right]}{\Omega}. \tag{195}$$

Concretely,

$$\begin{aligned}\sigma_{xx}(\Omega,T) &= v_x^2e^2\int\frac{d^2\mathbf{k}}{(2\pi)^2}\int_{-\infty}^{+\infty}\frac{d\omega_1}{\pi}\mathrm{Tr}\left[\sigma_1\mathrm{Im}\left[G^{\mathrm{ret}}_{\Delta}(\omega_1,\mathbf{k})\right]\sigma_1\mathrm{Im}\left[G^{\mathrm{ret}}_{\Delta}(\omega_1+\Omega,\mathbf{k})\right]\right]\\ &\times\frac{\left[n_F(\omega_1)-n_F(\omega_1+\Omega)\right]}{\Omega},\end{aligned} \tag{196}$$

$$\begin{aligned}\sigma_{yy}(\Omega,T) &= 9d_y^2e^2\int\frac{d^2\mathbf{k}}{(2\pi)^2}k_y^4\int_{-\infty}^{+\infty}\frac{d\omega_1}{\pi}\mathrm{Tr}\left[\sigma_2\mathrm{Im}\left[G^{\mathrm{ret}}_{\Delta}(\omega_1,\mathbf{k})\right]\sigma_2\mathrm{Im}\left[G^{\mathrm{ret}}_{\Delta}(\omega_1+\Omega,\mathbf{k})\right]\right]\\ &\times\frac{\left[n_F(\omega_1)-n_F(\omega_1+\Omega)\right]}{\Omega}.\end{aligned} \tag{197}$$

Substituting Eq. (149) and carrying out tedious derivations, we obtain

$$\begin{aligned}\sigma_{xx}(\Omega,T) &= \frac{\Gamma\left(\frac{7}{6}\right)}{8\sqrt[3]{2}\sqrt{\pi}\Gamma\left(\frac{2}{3}\right)}\frac{v_xe^2}{d_y^{\frac{1}{3}}}\frac{1}{\left(\Omega^2-4\Delta^2\right)^{\frac{1}{3}}}\left(1+12\frac{\Delta^2}{\Omega^2}\right)\theta\left(|\Omega|-2\Delta\right)\tanh\left(\frac{|\Omega|}{4T}\right)\\ &+\frac{3\Gamma\left(\frac{7}{6}\right)v_xe^2}{8\sqrt{\pi}\Gamma\left(\frac{2}{3}\right)d_y^{\frac{1}{3}}}\delta(\Omega)\frac{1}{T}\int_0^{+\infty}dE\frac{E^{\frac{7}{3}}}{E^2+\Delta^2}\frac{1}{\sinh^2\left(\frac{\sqrt{E^2+\Delta^2}}{2T}\right)},\end{aligned} \tag{198}$$

$$\begin{aligned}\sigma_{yy}(\Omega,T) &= \frac{9\Gamma\left(\frac{5}{6}\right)}{64\sqrt[3]{4}\sqrt{\pi}\Gamma\left(\frac{4}{3}\right)}\frac{d_y^{\frac{1}{3}}e^2}{v_x}\left(\Omega^2-4\Delta^2\right)^{\frac{1}{3}}\left(1+\frac{20}{3}\Delta^2\right)\theta\left(|\Omega|-2\Delta\right)\tanh\left(\frac{|\Omega|}{4T}\right)\\ &+\frac{15\Gamma\left(\frac{5}{6}\right)d_y^{\frac{1}{3}}e^2}{32\sqrt{\pi}\Gamma\left(\frac{4}{3}\right)v_x}\delta(\Omega)\frac{1}{T}\int_0^{+\infty}dE\frac{E^{\frac{11}{3}}}{E^2+\Delta^2}\frac{1}{\sinh^2\left(\frac{\sqrt{E^2+\Delta^2}}{2T}\right)}.\end{aligned} \tag{199}$$

The second terms in the right-hand side of Eqs. (198) and (199) represent the Drude peak

For $\Delta=0$, we have

$$\sigma_{xx}(\Omega,T) = \frac{\Gamma\left(\frac{7}{6}\right)}{8\sqrt[3]{2}\sqrt{\pi}\Gamma\left(\frac{2}{3}\right)}\frac{v_xe^2}{d_y^{\frac{1}{3}}}\frac{1}{|\Omega|^{\frac{2}{3}}}\tanh\left(\frac{|\Omega|}{4T}\right)+\frac{3\Gamma\left(\frac{7}{6}\right)}{8\sqrt{\pi}\Gamma\left(\frac{2}{3}\right)}\frac{v_xe^2}{d_y^{\frac{1}{3}}}\delta(\Omega)T^{\frac{1}{3}}\int_0^{+\infty}dx x^{\frac{1}{3}}\frac{1}{\sinh^2\left(\frac{x}{2}\right)}, \tag{200}$$

$$\sigma_{yy}(\Omega,T) = \frac{9\Gamma\left(\frac{5}{6}\right)}{64\sqrt[3]{4}\sqrt{\pi}\Gamma\left(\frac{4}{3}\right)}\frac{d_y^{\frac{1}{3}}e^2}{v_x}|\Omega|^{\frac{2}{3}}\tanh\left(\frac{|\Omega|}{4T}\right)+\frac{15\Gamma\left(\frac{5}{6}\right)}{32\sqrt{\pi}\Gamma\left(\frac{4}{3}\right)}\frac{d_y^{\frac{1}{3}}e^2}{v_x}\delta(\Omega)T^{\frac{5}{3}}\int_0^{+\infty}dx x^{\frac{5}{3}}\frac{1}{\sinh^2\left(\frac{x}{2}\right)}. \tag{201}$$

Taking $T=0$, we further obtain

$$\sigma_{xx}(\Omega,T) = \frac{\Gamma\left(\frac{7}{6}\right)}{8\sqrt[3]{2}\sqrt{\pi}\Gamma\left(\frac{2}{3}\right)}\frac{v_xe^2}{d_y^{\frac{1}{3}}}\frac{1}{|\Omega|^{\frac{2}{3}}}, \tag{202}$$

$$\sigma_{yy}(\Omega,T) = \frac{9\Gamma\left(\frac{5}{6}\right)}{64\sqrt[3]{4}\sqrt{\pi}\Gamma\left(\frac{4}{3}\right)}\frac{d_y^{\frac{1}{3}}e^2}{v_x}|\Omega|^{\frac{2}{3}}. \tag{203}$$

### E. Diamagnetic Susceptibility

For the case $\mathbf{B}=B\mathbf{e}_z$, the diamagnetic susceptibility is defined as

$$\chi_D = -e^2T\sum_{\omega_n}\int\frac{d^2\mathbf{k}}{(2\pi)^2}\mathrm{Tr}\left[\gamma_xG_{\Delta}(\omega_n,\mathbf{k})\gamma_yG_{\Delta}(\omega_n,\mathbf{k})\gamma_xG_{\Delta}(\omega_n,\mathbf{k})\gamma_yG_{\Delta}(\omega_n,\mathbf{k})\right]. \tag{204}$$

$\gamma_a$ is given by

$$\gamma_a = \frac{\partial \mathcal{H}_\Delta}{\partial k_a}, \tag{205}$$

with $a$ being the direction axis that is perpendicular to the direction of the magnetic field. Concretely

$$\gamma_x = \frac{\partial \mathcal{H}_\Delta}{\partial k_x} = v_x\sigma_1, \tag{206}$$

$$\gamma_y = \frac{\partial \mathcal{H}_\Delta}{\partial k_y} = 3d_y k_y^2\sigma_2. \tag{207}$$

Substituting the expressions of $\gamma_x$ and $\gamma_y$ into the expression $\chi_D$, we can get

$$\chi_D = -9v_x^2 d_y^2 e^2 T\sum_{\omega_n}\int\frac{d^2\mathbf{k}}{(2\pi)^2}k_y^4 \mathrm{Tr}\left[\sigma_1 G_0(\omega_n,\mathbf{k})\sigma_2 G_0(\omega_n,\mathbf{k})\sigma_1 G_0(\omega_n,\mathbf{k})\sigma_2 G_0(\omega_n,\mathbf{k})\right]. \tag{208}$$

Substituting Eq. (160) into Eq. (208), we obtain

$$\chi_D = 18v_x^2 d_y^2 e^2 T\int\frac{d^2\mathbf{k}}{(2\pi)^2}k_y^4\left(S_A - 8v_x^2k_x^2d_y^2k_y^6 S_B\right), \tag{209}$$

where

$$S_A = \sum_{\omega_n}\frac{1}{\left(\omega_n^2+E_{\mathbf{k}\Delta}^2\right)^2}, \tag{210}$$

$$S_B = \sum_{\omega_n}\frac{1}{\left(\omega_n^2+E_{\mathbf{k}\Delta}^2\right)^4}. \tag{211}$$

Performing the frequency summation, we obtain

$$S_A = \frac{1}{(2\pi T)^4}\frac{1}{2Y}\left[\frac{\pi}{Y^2}\tanh(\pi Y) - \frac{\pi^2}{Y}\frac{1}{\cosh^2(\pi Y)}\right], \tag{212}$$

$$S_B = \frac{1}{(2\pi T)^8}\frac{1}{48Y^3}\left[\frac{15\pi}{Y^4}\tanh(\pi Y) - \frac{15\pi^2}{Y^3}\frac{1}{\cosh^2(\pi Y)} - \frac{12\pi^3}{Y^2}\frac{\tanh(\pi Y)}{\cosh^2(\pi Y)} + \frac{2\pi^4}{Y}\frac{1}{\cosh^4(\pi Y)} - \frac{4\pi^4}{Y}\frac{\tanh^2(\pi Y)}{\cosh^2(\pi Y)}\right], \tag{213}$$

where

$$Y = \frac{E_{\mathbf{k}\Delta}}{2\pi T}. \tag{214}$$

Substituting Eqs. (212) and (213) into Eq. (209), employing the transformations Eqs. (153)-(157), and performing the integrations of $\delta$, we arrive

$$\chi_D = v_x d_y^{\frac{1}{3}} e^2 T^{-\frac{1}{3}} C_\chi, \tag{215}$$

where

$$C_\chi = \int_0^{+\infty} dx x^{\frac{5}{3}} \times\left\{\frac{1}{(x^2+\Delta'^2)}\left[\frac{1}{\sqrt{x^2+\Delta'^2}}\tanh\left(\sqrt{x^2+\Delta'^2}\right) - \frac{1}{\cosh^2\left(\sqrt{x^2+\Delta'^2}\right)}\right] - \frac{5}{112}\frac{x^4}{(x^2+\Delta'^2)^2}\left[\frac{15}{(x^2+\Delta'^2)^{\frac{3}{2}}}\tanh\left(\sqrt{x^2+\Delta'^2}\right) - \frac{15}{(x^2+\Delta'^2)}\frac{1}{\cosh^2\left(\sqrt{x^2+\Delta'^2}\right)} - \frac{12}{\sqrt{x^2+\Delta'^2}}\frac{\tanh\left(\sqrt{x^2+\Delta'^2}\right)}{\cosh^2\left(\sqrt{x^2+\Delta'^2}\right)} + 2\frac{1}{\cosh^4\left(\sqrt{x^2+\Delta'^2}\right)} - 4\frac{\tanh^2\left(\sqrt{x^2+\Delta'^2}\right)}{\cosh^2\left(\sqrt{x^2+\Delta'^2}\right)}\right]\right\}, \tag{216}$$

with $\Delta' = \frac{\Delta}{2T}$.

For $\Delta = 0$, we have

$$C_\chi = \frac{3\Gamma\left(\frac{5}{6}\right)}{4\sqrt[3]{2}\pi^{\frac{3}{2}}\Gamma\left(\frac{4}{3}\right)}\int_0^{+\infty} dx x^{\frac{5}{3}}\left\{\frac{1}{x^2}\left[\frac{1}{x}\tanh(x) - \frac{1}{\cosh^2(x)}\right] - \frac{5}{112}\right.$$
$$\left.\times\left[\frac{15}{x^3}\tanh(x) - \frac{15}{x^2}\frac{1}{\cosh^2(x)} - \frac{12}{x}\frac{\tanh(x)}{\cosh^2(x)} + 2\frac{1}{\cosh^4(x)} - 4\frac{\tanh^2(x)}{\cosh^2(x)}\right]\right\}$$
$$\approx 0.172765. \tag{217}$$

Thus,

$$\chi_D = v_x d_y^{\frac{1}{3}} e^2 T^{-\frac{1}{3}} C_\chi \propto T^{-\frac{1}{3}}. \tag{218}$$

For finite $\Delta$, in the limit $T \ll \Delta$, from numerical conclusion, we find that $C_\chi$ can be approximately by

$$C_\chi \propto \frac{\tanh(\Delta')}{\Delta'^{\frac{1}{3}}} \propto \frac{\tanh\left(\frac{\Delta}{2T}\right)}{\left(\frac{\Delta}{2T}\right)^{\frac{1}{3}}} \propto \frac{1}{\left(\frac{\Delta}{2T}\right)^{\frac{1}{3}}}. \tag{219}$$

Thus, in the low temperature regime, $\chi_D$ can be expressed by

$$\chi_D \propto T^{-\frac{1}{3}}\frac{1}{\left(\frac{\Delta}{2T}\right)^{\frac{1}{3}}} \propto \frac{1}{\Delta^{\frac{1}{3}}}. \tag{220}$$

### F. Quantum anomalous Hall Effect

The Hamiltonian is given by

$$\mathcal{H}_\Delta = d_x\sigma_x + d_y\sigma_y + d_z\sigma_z$$
$$= v_x k_x \sigma_x + d_y k_y^3 \sigma_y + \Delta\sigma_z. \tag{221}$$

The vector $\mathbf{D}$ is defined as

$$\mathbf{D} = D_x\mathbf{e}_x + D_y\mathbf{e}_y + D_z\mathbf{e}_z$$
$$= v_x k_x \mathbf{e}_x + d_y k_y^3 \mathbf{e}_y + \Delta\mathbf{e}_z. \tag{222}$$

The unit vector takes the form

$$\hat{\mathbf{D}} = \frac{\mathbf{D}}{|\mathbf{D}|} = \frac{v_x k_x \mathbf{e}_x + d_y k_y^3 \mathbf{e}_y + \Delta\mathbf{e}_z}{\sqrt{v_x^2 k_x^2 + d_y^2 k_y^6 + \Delta^2}}. \tag{223}$$

The corresponding Chern number is given by

$$C = \frac{1}{4\pi}\int d^2\mathbf{k}\left(\frac{\partial\hat{\mathbf{D}}}{\partial k_x}\times\frac{\partial\hat{\mathbf{D}}}{\partial k_y}\right)\cdot\hat{\mathbf{D}}. \tag{224}$$

Substituting the expression of $\hat{\mathbf{D}}$, we can get

$$C = \frac{1}{4\pi}\int d^2\mathbf{k}\frac{3v_x d_y k_y^2\Delta}{\left[v_x^2k_x^2 + d_y^2k_y^6 + \Delta^2\right]^{\frac{3}{2}}}$$
$$= \frac{1}{\pi}3v_x d_y\Delta\int_0^{+\infty}\int_0^{+\infty} dk_x dk_y \frac{k_y^2}{\left[v_x^2k_x^2 + d_y^2k_y^6 + \Delta^2\right]^{\frac{3}{2}}}. \tag{225}$$

Utilizing the transformations Eqs. (153)-(157), we obtain

$$\begin{aligned} C &= \frac{1}{\pi}\frac{v_x}{|v_x|}\frac{d_y}{|d_y|}\Delta\int_0^{+\infty}dE\frac{E}{[E^2+\Delta^2]^{\frac{3}{2}}}\int_0^{+\infty}d\xi\frac{1}{(1+\xi^2)} \\ &= \frac{1}{2}\mathrm{sgn}(v_x)\mathrm{sgn}(d_y)\mathrm{sgn}(\Delta). \end{aligned} \tag{226}$$

Thus, the system has a quantized anomalous Hall conductivity

$$\sigma_{xy} = C\frac{e^2}{h}, \tag{227}$$

where $h$ is the Planck constant.

## VII. SHORT-RANGE FOUR-FERMION INTERACTION

Taking the short-range four-fermion interaction $g_3\left(\psi^\dagger\sigma_3\psi\right)^2$ as an example, we show the details of derivation and calculation for the mean-field analysis.

### A. Derivation for the self-consistent equation

Under the influence of short-range four-fermion interaction $g_3\left(\psi^\dagger\sigma_3\psi\right)^2$, the expectation value

$$\Delta = \left\langle\psi^\dagger\sigma_3\psi\right\rangle, \tag{228}$$

could become finite. Considering the order parameter $\Delta$, the fermion propagator can be written as

$$G(\omega,\mathbf{k},\Delta) = \frac{1}{-i\omega+v_xk_x\sigma_1+d_yk_y^3\sigma_2+\Delta\sigma_3} \tag{229}$$

For finite temperature, we employ the propagator in Matsubara formalism as following

$$G(\omega_n,\mathbf{k},\Delta) = \frac{1}{-i\omega_n+v_xk_x\sigma_1+d_yk_y^3\sigma_2+\Delta\sigma_3}, \tag{230}$$

where $\omega_n = (2n+1)\pi T$ with $n$ being integers.

The partition functions is [9]

$$\begin{aligned} Z &= \int\mathcal{D}i\psi^\dagger\mathcal{D}\psi e^{S} \\ &= \prod_{\omega_n}\prod_{\mathbf{k}}\int\mathcal{D}i\psi^\dagger\mathcal{D}\psi e^{i\psi^\dagger_{\omega_n,\mathbf{k}}(-i)\beta G^{-1}(\omega_n,\mathbf{k},\Delta)\psi_{\omega_n,\mathbf{k}}-\int d\tau\int d^2\mathbf{x}\frac{\Delta^2}{2g_3}}, \end{aligned} \tag{231}$$

where $\beta = \frac{1}{T}$. Using the functional integral formula

$$\int\mathcal{D}\eta^\dagger\mathcal{D}\eta e^{\eta^\dagger K\eta} = \det K, \tag{232}$$

we get

$$Z = \prod_{\omega_n}\prod_{\mathbf{k}}\beta^2\det\left[(-i)G^{-1}(\omega_n,\mathbf{k},\Delta)\right]e^{-\int d\tau\int d^2\mathbf{x}\frac{\Delta^2}{2g_3}}, \tag{233}$$

which can be further written as

$$\ln Z = \sum_{\omega_n}\sum_{\mathbf{k}}\ln\left(\beta^2\det\left[(-i)G^{-1}(\omega_n,\mathbf{k},\Delta)\right]\right)-\int d\tau\int d^2\mathbf{x}\frac{\Delta^2}{2g_3}. \tag{234}$$

It is easy to verify that

$$\det\left[(-i)G^{-1}(\omega_n,\mathbf{k},\Delta)\right] = \omega_n^2 + E_{\mathbf{k},\Delta}^2, \tag{235}$$

where

$$E_{\mathbf{k},\Delta} = \sqrt{v_x^2 k_x^2 + d_y^2 k_y^6 + \Delta^2}. \tag{236}$$

Thus we obtain

$$\ln Z = \sum_{\omega_n}\sum_{\mathbf{k}} \ln\left(\beta^2\left(\omega_n^2 + E_{\mathbf{k},\Delta}^2\right)\right) - \int d\tau \int d^2\mathbf{x}\frac{1}{2g_3}\Delta^2. \tag{237}$$

Carrying out the summation of frequency, we arrive

$$\begin{aligned}\ln Z &= \sum_{\mathbf{k}}\left[\frac{1}{T}E_{\mathbf{k},\Delta} + 2\ln\left(1+e^{-\frac{E_{\mathbf{k},\Delta}}{T}}\right)\right] - \int d\tau\int d^2\mathbf{x}\frac{1}{2g_3}\Delta^2 \\ &= \mathcal{V}\int\frac{d^2\mathbf{k}}{(2\pi)^2}\left[\frac{1}{T}E_{\mathbf{k},\Delta} + 2\ln\left(1+e^{-\frac{E_{\mathbf{k},\Delta}}{T}}\right)\right] - \beta\mathcal{V}\frac{1}{2g_3}\Delta^2,\end{aligned} \tag{238}$$

where $\mathcal{V}$ is volume of sample. We have used the replacement

$$\frac{1}{\mathcal{V}}\sum_{\mathbf{k}} \to \int\frac{d^2\mathbf{k}}{(2\pi)^2}. \tag{239}$$

The free energy density $f$ and free energy are defined as

$$\begin{aligned}f &= \frac{F}{\mathcal{V}} = -\frac{1}{\beta}\ln Z \\ &= -2T\int\frac{d^2\mathbf{k}}{(2\pi)^2}\ln\left(2\cosh\left(\frac{E_{\mathbf{k},\Delta}}{2T}\right)\right) + \frac{1}{2g_3}\Delta^2.\end{aligned} \tag{240}$$

The self-consistent gap equation is determined by

$$\frac{\partial f}{\partial\Delta} = 0, \tag{241}$$

which leads the self-consistent equation

$$1 = g_3\int\frac{d^2\mathbf{k}}{(2\pi)^2}\tanh\left(\frac{E_{\mathbf{k},\Delta}}{2T}\right)\frac{1}{E_{\mathbf{k},\Delta}}. \tag{242}$$

At zero temperature, the equation becomes

$$1 = g_3\int\frac{d^2\mathbf{k}}{(2\pi)^2}\frac{1}{E_{\mathbf{k},\Delta}}. \tag{243}$$

## B. Solving the self-consistent equation

### *1. Zero temperature*

At zero temperature, the self-consistent equations can be written as

$$1 = g_3\int\frac{d^2\mathbf{k}}{(2\pi)^2}\frac{1}{\sqrt{v_x^2 d_x^2 + d_y^2 k_y^6 + \Delta^2}} \tag{244}$$

$$= g_3\frac{1}{\pi^2}\int_0^{+\infty}\int_0^{+\infty} dk_x dk_y\frac{1}{\sqrt{v_x^2 d_x^2 + d_y^2 k_y^6 + \Delta^2}}. \tag{245}$$

Using the transformations Eqs. (153)-(157), we arrive

$$\begin{aligned}1 &= g_3\frac{1}{3\pi^2 v_x d_y^{\frac{1}{3}}}\int_0^{\Lambda} dE\frac{E^{\frac{1}{3}}}{\sqrt{E^2+\Delta^2}}\int_0^{+\infty} d\xi\frac{1}{\xi^{\frac{2}{3}}\left(1+\xi^2\right)^{\frac{2}{3}}} \\ &= g_3\frac{\Gamma\left(\frac{7}{6}\right)}{\pi^{\frac{3}{2}}\Gamma\left(\frac{2}{3}\right)v_x d_y^{\frac{1}{3}}}\int_0^{\Lambda} dE\frac{E^{\frac{1}{3}}}{\sqrt{E^2+\Delta^2}}. \end{aligned} \tag{246}$$

It can be further written as

$$1 = g_3\frac{\Gamma\left(\frac{7}{6}\right)}{\pi^{\frac{3}{2}}\Gamma\left(\frac{2}{3}\right)v_x d_y^{\frac{1}{3}}}\left[\Lambda^{\frac{1}{3}}\int_0^1 dx\left(\frac{x^{\frac{1}{3}}}{\sqrt{x^2+\left(\frac{\Delta}{\Lambda}\right)^2}}-x^{-\frac{2}{3}}\right)+3\Lambda^{\frac{1}{3}}\right]. \tag{247}$$

Taking $\Delta = 0$, we get the critical coupling strength $g_{3c}$ which satisfies

$$g_{3c} = \frac{\pi^{\frac{3}{2}}\Gamma\left(\frac{2}{3}\right)v_x d_y^{\frac{1}{3}}}{3\Gamma\left(\frac{7}{6}\right)\Lambda^{\frac{1}{3}}}. \tag{248}$$

In the limit $\Delta \ll \Lambda$, we have

$$1 = \frac{3\Gamma\left(\frac{7}{6}\right)g_3\Lambda^{\frac{1}{3}}}{\pi^{\frac{3}{2}}\Gamma\left(\frac{2}{3}\right)v_x d_y^{\frac{1}{3}}}\left[1-\frac{3\Gamma\left(\frac{5}{3}\right)\Gamma\left(\frac{5}{6}\right)}{2\sqrt{\pi}}\left(\frac{\Delta}{\Lambda}\right)^{\frac{1}{3}}\right] \tag{249}$$

$$= \frac{g_3}{g_{3c}}\left[1-\frac{3\Gamma\left(\frac{5}{3}\right)\Gamma\left(\frac{5}{6}\right)}{2\sqrt{\pi}}\left(\frac{\Delta}{\Lambda}\right)^{\frac{1}{3}}\right] \tag{250}$$

Thus $\Delta$ is given by

$$\Delta \approx b_1\frac{\left(g_3-g_{3c}\right)^3}{g_{3c}^3}, \tag{251}$$

where

$$b_1 = \left[\frac{2\sqrt{\pi}}{3\Gamma\left(\frac{5}{3}\right)\Gamma\left(\frac{5}{6}\right)}\right]^3 \approx 1.55926. \tag{252}$$

### *2. Finite temperature*

At finite temperature, the self-consistent equation can be written as

$$\begin{aligned}\frac{1}{g_3} &= \int\frac{d^2\mathbf{k}}{(2\pi)^2}\frac{1}{\sqrt{v_x^2d_x^2+d_y^2k_y^6+\Delta^2}}\tanh\left(\frac{\sqrt{v_x^2d_x^2+d_y^2k_y^6+\Delta^2}}{2T}\right) \\ &= \frac{1}{\pi^2}\int_0^{+\infty}\int_0^{+\infty}dk_xdk_y\frac{1}{\sqrt{v_x^2d_x^2+d_y^2k_y^6+\Delta^2}}\tanh\left(\frac{\sqrt{v_x^2d_x^2+d_y^2k_y^6+\Delta^2}}{2T}\right). \end{aligned} \tag{253}$$

Using the transformations Eqs. (153)-(157), we get

$$\begin{aligned}\frac{1}{g_3} &= \frac{1}{3\pi^2 v_x d_y^{\frac{1}{3}}}\int dE\frac{E^{\frac{1}{3}}}{\sqrt{E^2+\Delta^2}}\tanh\left(\frac{\sqrt{E^2+\Delta^2}}{2T}\right)\int d\xi\frac{1}{\xi^{\frac{2}{3}}\left(1+\xi^2\right)^{\frac{2}{3}}} \\ &= \frac{\Gamma\left(\frac{7}{6}\right)}{\pi^{\frac{3}{2}}\Gamma\left(\frac{2}{3}\right)v_x d_y^{\frac{1}{3}}}\int_0^{\Lambda} dE\frac{E^{\frac{1}{3}}}{\sqrt{E^2+\Delta^2}}\tanh\left(\frac{\sqrt{E^2+\Delta^2}}{2T}\right). \end{aligned} \tag{254}$$

$T_c$ is determined by

$$\frac{1}{g_3} = \frac{\Gamma\left(\frac{7}{6}\right)}{\pi^{\frac{3}{2}}\Gamma\left(\frac{2}{3}\right)v_x d_y^{\frac{1}{3}}}\int_0^{\Lambda} dE E^{-\frac{2}{3}}\tanh\left(\frac{E}{2T_c}\right)$$
$$= \frac{2^{\frac{1}{3}}\Gamma\left(\frac{7}{6}\right)T_c^{\frac{1}{3}}}{\pi^{\frac{3}{2}}\Gamma\left(\frac{2}{3}\right)v_x d_y^{\frac{1}{3}}}\left[3\left(\frac{\Lambda}{2T_c}\right)^{\frac{1}{3}}\tanh\left(\frac{\Lambda}{2T_c}\right) - 3\int_0^{\frac{\Lambda}{2T_c}} dx x^{\frac{1}{3}}\frac{1}{\cosh^2(x)}\right]. \quad (255)$$

If $T_c \ll \Lambda$, the equation can be further written as

$$\frac{1}{g_3} = \frac{2^{\frac{1}{3}}\Gamma\left(\frac{7}{6}\right)T_c^{\frac{1}{3}}}{\pi^{\frac{3}{2}}\Gamma\left(\frac{2}{3}\right)v_x d_y^{\frac{1}{3}}}\left[3\left(\frac{\Lambda}{2T_c}\right)^{\frac{1}{3}} - 3\int_0^{+\infty} dx x^{\frac{1}{3}}\frac{1}{\cosh^2(x)}\right]$$
$$= \frac{1}{g_{3c}} - \sqrt[3]{2}a\frac{1}{g_{3c}}\left(\frac{T_c}{\Lambda}\right)^{\frac{1}{3}}, \quad (256)$$

where

$$a = \int_0^{+\infty} dx x^{\frac{1}{3}}\frac{1}{\cosh^2(x)} \approx 0.810469. \quad (257)$$

Then $T_c$ can be expressed by

$$T_c \approx b_2\Lambda\frac{(g_3 - g_{3c})^3}{g_{3c}^3}, \quad (258)$$

where

$$b_2 = \frac{1}{2a^3} \approx 0.939205. \quad (259)$$


[1] P. Maris, Influence of the full vertex and vacuum polarization on the fermion propagator in (2+1)-dimensional QED, Phys. Rev. D **54**, 5049 (1996).
[2] J.-R. Wang and G.-Z. Liu, Absence of dynamical gap generation in suspended graphene, New J. Phys. **14**, 043036 (2012).
[3] M. E. Carrington, C. S. Fischer, L. von Smekal, and M. H. Thoma, Dynamical gap generation in graphene with frequency-dependent renormalization effects, Phys. Rev. B **94**, 125102 (2016).
[4] M. E. Carrington, C. S. Fischer, L. von Smekel, and M. H. Thoma, Role of frequency dependence in dynamical gap generation in graphene, Phys. Rev. B **97**, 115411 (2018).
[5] D. V. Khveshchenko, Ghost excitonic insulator transition in layered graphite, Phys. Rev. Lett. **87**, 246802 (2001).
[6] E. V. Gorbar, V. P. Gusynin, V. A. Miransky, I. A. Shovkovy, Magnetic field driven metal-insulator phase transition in planar systems, Phys. Rev. B **66**, 045108 (2002).
[7] G.-Z. Liu, W. Li, and G. Cheng, Interaction and excitonic insulating transition in graphene, Phys. Rev. B **79**, 205429 (2009).
[8] J.-R. Wang, G.-Z. Liu, and C.-J. Zhang, Excitonic pairing and insulating transition in two-dimensional semi-Dirac semimetals, Phys. Rev. B **95**, 075129 (2017).
[9] J. I. Kapusta and C. Gale, *Finite-Temperature Field Theory: Principles and Applications* (Cambridge University Press, UK; New York,2006).
